# Supplementary material for: Near-Optimal Procedures for Model Discrimination with Non-Disclosure Properties
Source: arXiv:2012.02901 source file (2021-07-10)
Supplement: Supplementary file 1 [file appendix.tex]

%\section{Upper bounds for linear model}

%\subsection{Proof of Proposition~\ref{prop:upper-fixed-design}}

\section{Proof of Theorem~\ref{th:upper-random-design}}
\label{app:upper-linear}

Let~$\wh S = \wh S_0 - \wh S_1$ be the statistic whose sign is examined in~$\wh T$, i.e.,~$\wh T = \ind\{\wh S_0 \ge \wh S_1 \}$. Note that~$\wh r_0 := \rank(\wh\bSigma_0) = \rank(\bPi_X)$ and~$\wh r_1 := \rank(\wh\bSigma_1) = \rank(\bPi_{\wt X})$. Observe that~$\wh r_k = \min[n_k, r_k]$~a.s.
Let also~$\xi, \wt \xi$ be defined as in the proof of Proposition~\ref{prop:upper-fixed-design}.
Now, under~$\cH_0$ we have
\[
\wh S_0 = \|\bPi_{X} \xi\|^2 - \rank(\bPi_{X}) = \|\bPi_{X} \xi\|^2 - \wh r_0.
\]
Clearly,~$\|\bPi_{X} \xi\|^2 \sim \chi_{\wh r_0}^2$ conditionally on~$X$ since~$\xi$ is independent of~$X$. Similarly,
\[
\begin{aligned}
\wh S_1 &= \|\bPi_{\wt X} [\wt\xi  + \wt X (\theta_1 - \theta_0)]\|^2 - \rank(\bPi_{\wt X}) \\
        &= \|\bPi_{\wt X} \wt \xi\|^2 - \wh r_1 + \|\wt X (\theta_1 - \theta_0)\|^2 + 2 \langle \wt \xi, \wt X (\theta_1 - \theta_0) \rangle\\
        &= \|\bPi_{\wt X} \wt \xi\|^2 - \wh r_1 + n_1 \wh \Delta_1^2 + 2\langle \wt \xi, \wt X(\theta_1-\theta_0)\rangle \\
        &= \wh S_1^o + n_1 \wh \Delta_1^2 + 2\wt\zeta,
\end{aligned}
\]
where we defined~$\wh S_1^o := \|\bPi_{\wt X} \wt \xi\|^2 - \wh r_1$, distributed as~$\chi_{\wh r_1}^2$ conditionally on~$\wt X$, and~$\wt \zeta := \langle \wt \xi, \wt X(\theta_1-\theta_0)\rangle$, distributed as~$\cN(0,n_1\wh \Delta_1^2)$ conditionally on~$\wt X$. Using tail bounds~\eqref{eq:tail-bounds}, we get
% Observe that~$\langle \wt \xi, \wt X(\theta_1-\theta_0)\rangle \sim \cN(0,n_1\wh\Delta_1^2)$ conditionally to~$\wt X$. 
% and it concentrates roughly as~$\sqrt{n_1}\Delta_1 |\chi_1^2 - 1|$  when marginalized over~$\wt X$. 
% On the other hand, by~\cite[Lemma~1]{laurent2000adaptive} we have
% Hence, 
\[
\begin{aligned}
\Prob_{\cH_0}[\wh S > 0|X,\wt X] 
% = \Prob[\wh S_0 - \wh S_1^o + 2z \ge n_1 \wh \Delta_1^2] 
&\le \Prob\bigg[\wh S_0 \ge \frac{n_1 \wh \Delta_1^2}{3} \; \bigg| \; X,\wt X \bigg] 
	+ \Prob\bigg[-\wh S_1^o \ge  \frac{n_1 \wh\Delta_1^2}{3} \; \bigg| \; \wt X \bigg] 
	+ \Prob\bigg[\wt\zeta \ge \frac{n_1 \wh \Delta_1^2}{6} \; \bigg| \; \wt X\bigg] \\
&\le 2\exp(-c n_1 \wh \Delta_1^2 ) 
    +2\exp\bigg(-\frac{c n_1^2 \wh \Delta_1^4}{\wh r_0 \vee \wh r_1} \bigg) 
= 2\exp (-c n_1 \wh \Delta_1^2 ) 
    +2\exp\bigg(-\frac{c n_1^2 \wh \Delta_1^4}{\bar r} \bigg),
\end{aligned}
\]
where in the final transition we used that~$\bar r := \min(n_0, r_0) \vee \min(n_1, r_1) = \wh r_0 \vee \wh r_1$ almost surely.
% Conditioned on~$\wt X$, 
% \[
% \Prob_0[\wh S > 0 | \wt X]  
% \le \exp\left(-\alpha_0 n_1 \wh \Delta_1^2 \right) 
%     +\exp\left(-\frac{\alpha_0^2 n_1^2 \wh \Delta_1^4}{2d_0} \right) 
%     +\exp\left(-\frac{\alpha_1^2 n_1^2 \wh \Delta_1^4}{2d_1} \right) 
%     +\Prob[z \ge \frac{\gamma}{2} n_1 \wh \Delta_1^2].
% \]
%%
% We choose~$\gamma = 1/3 = \alpha_0 = \alpha_1$.
% and~$\alpha_0, \alpha_1$ to equalize the two middle terms:
% \[
% \begin{aligned}
% 2\alpha_0 &= \frac{\sqrt{d_0}}{\sqrt{d_0} + \sqrt{d_1}}, \quad 
% 2\alpha_1  = \frac{\sqrt{d_1}}{\sqrt{d_0} + \sqrt{d_1}}.
% \end{aligned}
% \]
% (OK, We can just put uniform weights in fact...). 
%%
% Conditionally on~$\wt X$ we get
% \[
% \begin{aligned}
% \Prob_0[\wh S > 0 | \wt X]  
% \le \exp\left(-c n_1 \wh \Delta_1^2 \right) 
%     +2\exp\left(-\frac{c n_1^2 \wh \Delta_1^4}{\max(d_0, d_1)} \right) 
%     +\exp[-c' n_1 \wh \Delta_1^2] \\ 
% \le 2\exp\left(-c n_1 \wh \Delta_1^2 \right) 
%     +2\exp\left(-\frac{c n_1^2 \wh \Delta_1^4}{\max(d_0, d_1)} \right).
% \end{aligned}
% \]
% where the last term is due to the standard Gaussian tail bound. 
It remains to take expectation over~$X,\wt X$.
To this end, observe that
\[
\wh \Delta_1^2 = \frac{1}{n_1} \sum_{i=1}^{n_1} \lang \wt x_i, \theta_1 - \theta_0 \rang^2,
\]
where~$\wt x_i \sim \cN(0,\bSigma_1)$ and are~i.i.d. Hence,
$
n_1\wh \Delta_1^2/\Delta_1^2 \sim \chi_{n_1}^2.
$
By~\eqref{eq:tail-bounds-chi-sq-left}, this gives
\[
\Prob \left[ n_1\wh \Delta_1^2 \le {n_1 \Delta_1^2}/{2} \right] \le \exp(-cn_1). 
\]
Thus, we arrive at
$
\Prob_{\cH_0}[\wh S > 0] \le \exp(-cn_1) + 2\exp\left(-c n_1 \Delta_1^2 \right) 
    +2\exp\left(-{c n_1^2 \Delta_1^4}/{\bar r}\right)
$
as claimed.
% Note that the first term is dominated by the second one when~$\Delta_1 \lsim 1$ (which is a mild condition).
\qed

\section{Proof of Theorem~\ref{th:lower-gaussian}}

\label{app:lower} 

Our goal in this section is to prove Theorem~\ref{th:lower-gaussian}. 
We proceed in four steps deferred to Sec.~\ref{sec:lower-fixed-design-reduction}--\ref{sec:lower-orths}.

\subsection{Reduction to fixed-design setup}

\label{sec:lower-fixed-design-reduction}

%In this section, our final goal is to derive a matching lower bound for the minimax testing error in the case of a well-specified linear model. 
We first show that one can pass to the fixed-design setup, proving the following bound: 
% to the random design setup will follow from the law of total expectation, through an %argument similar to the one that will be used later on when proving Theorem~\ref{th:upper-random-design} (see Appendix~\ref{app:upper}).
%Let~$\Delta^2 > 0$ be arbitrary. 
%With fixed design, our goal is to prove the bound
\begin{equation}
\label{eq:lower-fixed-design}
\underset{T}{\inf} \underset{(\theta_0,\theta_1) \in \wh \Theta}{\sup} 
\left\{ \Prob_{\cH_0}[T = 1|X,\tilde{X}] + \Prob_{\cH_1}[T = 0|X,\tilde{X}] \right\}
\ge  
C \exp \left(-c n^{\vphantom 2} \Delta^2 \min\left[1, \frac{n^{\vphantom 2}\Delta^2}{\wh\rmin}\right]\right),
\end{equation}
the infinum being over all measurable maps~$(\theta^*, X,Y,\wt X, \wt Y) \to \{0,1\}$ as in~\eqref{eq:lower-gaussian}, the supremum over
\begin{equation}
\label{def:set-empirical}
\wh \Theta = \wh \Theta(32\Delta^2) := \{(\theta_0,\theta_1): \max[\wh \Delta_0^2, \wh \Delta_1^2] \geq 32\Delta^2\}
\end{equation} 
for~$\wh \Delta_{0}^2,\wh \Delta_{1}^2$ defined in~\eqref{def:Delta-empirical}, and ~$\wh\rmin := \rank(\wh \bSigma_0) \wedge \rank(\wh \bSigma_1)$ with~$\wh \bSigma_0 = \frac{1}{n} X^\top X$ and~$\wh \bSigma_1 = \frac{1}{n} \wt X^\top \wt X$. 
Moreover, we will make one additional assumption that the matrices~$\wh \bSigma_0$ and~$\wh \bSigma_1$ commute. To obtain~\eqref{eq:lower-gaussian}, we will then construct two design distributions~$\cD_0,\cD_1$ as in the premise of the theorem, such that the corresponding (mutually independent) sample covariances~$\wh\bSigma_0, \wh\bSigma_1$ commute a.s., and
\[
\rmin/4 \le \wh \rmin \le \rmin
\]
with probability~$\ge 1/8$, where~$\rmin = \min [r_0, r_1, n]$.  
When combined with~\eqref{eq:lower-fixed-design}, this will readily yield~\eqref{eq:lower-gaussian}.
Indeed, by Markov's inequality~$\wh \Delta_0^2 \le 32\Delta_0^2$ and~$\wh \Delta_1^2 \le 32\Delta_1^2$ simultaneously with probability~$\ge 15/16$ over~$(X, \wt X)$. 
Under the joint event (holding with probability~$\ge 1-7/8-1/16 = 1/16$), one has~$\wh\Theta(32\Delta^2) \subseteq \Theta(\Delta^2)$, i.e., the supremum in~\eqref{eq:lower-gaussian} is over the larger set; thus, %one can lower-bound the left-hand side~\eqref{eq:lower-gaussian} as follows
\[
\begin{aligned}
&\underset{T}{\inf} \underset{(\theta_0,\theta_1) \in \Theta(\Delta^2)}{\sup} 
\left\{ \Prob_{\cH_0}[T = 1] + \Prob_{\cH_1}[T = 0] \right\} \\
\ge 
&\frac{1}{16} \underset{T}{\inf} \underset{(\theta_0,\theta_1) \in \wh \Theta(32\Delta^2)}{\sup} 
\left\{ \Prob_{\cH_0}[T = 1|X,\tilde{X}] + \Prob_{\cH_1}[T = 0|X,\tilde{X}] \right\} 
\ge
\frac{C}{16} \exp \left(-c n^{\vphantom 2} \Delta^2 \min\left[1, \frac{4n^{\vphantom 2}\Delta^2}{\rmin}\right]\right),
\end{aligned}
\]
%on the event in which~\eqref{eq:lower-fixed-design} holds with~$\rmin/4 \le \wh \rmin \le \rmin$, 
which is~\eqref{eq:lower-gaussian}. 
Thus, we can indeed focus on proving~\eqref{eq:lower-fixed-design} assuming that~$\wh\bSigma_0$ and~$\wh\bSigma_1$ commute. We do this in Sec.~\ref{sec:lower-easy}-\ref{sec:lower-hard}; then in Sec.~\ref{sec:lower-orths} we construct distributions~$\cD_0, \cD_1$ with required properties. 

Note that~\eqref{eq:lower-fixed-design} comprises two bounds simultaneously: rank-independent bound~$\exp(-cn\Delta^2)$ and the bound depending on~$\wh\rmin$.
We first prove the rank-independent bound (Sec.~\ref{sec:lower-easy}), and then extend the analysis to capture the dependency on~$\rmin$ (Sec.~\ref{sec:lower-hard}). 
In fact, as we are about to see, for the first bound it suffices to consider a further simplified testing problem in which {\em Auditor is shown both models~$\{\theta_0, \theta_1\}$ up to a permutation,} rather than just~$\theta^*$.  
However, capturing the dependency on~$\rmin$ requires to take into account that one of the two models is unknown, and put a suitable prior on it.
%We now introduce the simpler testing problem.

\subsection{Rank-independent bound}
\label{sec:lower-easy}
Let~$\bar{\theta} := \theta_0 + \theta_1 - \theta^*$, so that~$\{\theta_*, \bar\theta\} = \{\theta_0, \theta_1\}$ as the two sets regardless of the hypothesis. 
Now, observe that the two hypotheses~$\cH_0: \theta_0 = \theta^*$ and~$\cH_1: \theta_1 = \theta^*$ can be reformulated as the hypotheses~$(\theta_0, \theta_1) = (\theta^*, \bar\theta)$
and~$(\theta_0, \theta_1) = (\bar\theta, \theta^*)$
about the aggregated parameter~$(\theta_0, \theta_1)$. 
%The sum of error probabilities of two types in~\eqref{eq:lower-fixed-design} corresponds to taking the 
%This would allow us to apply the Neyman-Pearson lemma if~$\cH_0, \cH_1$ were two {\em simple} hypotheses about 
Since~$\bar\theta$ is unknown, we are dealing with a composite testing problem, and thus cannot apply the Neyman-Pearson lemma. To put us in the two-point hypothesis testing situation, we can simply fix a value of~$\bar\theta$, and assume that it is also known -- in other words, consider the following testing problem:
\begin{equation}
\label{eq:two-point-problem}
\boxed{
\begin{aligned}
\textit{Given the data}\;
&n,\wh r_0, \wh r_1,(\theta^*, \bar\theta) \in \wh\Theta, \; 
(X,Y) \in \Prob_0^{\otimes n},\; (\wt X,\wt Y) \sim \Prob_1^{\otimes n},\;
\textit{test}\\
&\bar\cH_0: (\theta^*, \bar\theta) = (\theta_0, \theta_1) \; \text{vs.} \;
\bar\cH_1:  (\theta^*, \bar\theta) = (\theta_1, \theta_0).
\end{aligned}}
\tag{$\cP^o$}
\end{equation}
Clearly,~\eqref{eq:two-point-problem} is a problem of testing between two {\em simple} hypotheses about the unknown parameter~$(\theta_0, \theta_1) \in \wh\Theta(\Delta^2)$. 
Hence, by the Neyman-Pearson lemma, the sum of type I and type II error probabilities of any test for~\eqref{eq:two-point-problem} is lower-bounded by that for the likelyhood-ratio test, as given by
\begin{equation}
\label{eq:test-oracle}
T_{LR} = \ind\{  \| Y - X\theta^*\|^2 + \| \tilde{Y} - \tilde{X} \bar\theta\|^2 \geq \| Y - X\bar\theta\|^2 + \| \tilde{Y} - \tilde{X} \theta^*\|^2\}.
\end{equation}
On the other hand,~\eqref{eq:two-point-problem} cannot be harder than the initial testing problem considered in~\eqref{eq:lower-fixed-design}. 
Indeed, each test admissible in~\eqref{eq:lower-fixed-design}
can also be understood as a mapping~$(\theta^*, \bar \theta,X,Y, \wt X,\wt Y) \to \{0,1\}$ that does {\em not} depend on~$\bar \theta$, whereas in~$\cP^o$ one is also allowed to use the tests that do depend on~$\bar \theta$ and thus are not~$(\theta^*,X,Y,\wt X,\wt Y)$-measurable. 
Thus, we can bound the left-hand side of~\eqref{eq:lower-fixed-design} as follows:
% are not allowed to use~$\bar\theta$, so the set of all such tests is contained in the set of all admissible tests in~\eqref{eq:two-point-problem} ``projected'' on the restricted data~$(\theta^*, X, Y, \wt X, \wt Y)$.
% in turn, this is equivalent to sampling the ordered pair~$(\theta^{*},\bar \theta)$ uniformly over the two permutations of~$(\theta_0,\theta_1)$. 
%%
%Let~$(\theta_0,\theta_1)$ be on the boundary of~$\wh\Theta(\Delta^2)$, i.e.,~$\max [\wh \Delta_0^2, \wh \Delta_1^2] = \Delta^2$. 
% consider first the simplified testing problem as follows:
%%
%Applying the Neyman-Pearson lemma to the above testing problem, we conclude that
\[
\begin{aligned}
\underset{T: (\theta^*,X,Y,\wt X,\wt Y) \to \{0,1\}}{\inf} \;
	&\underset{(\theta_0, \theta_1) \in \wh\Theta}{\sup} 
\left\{\Prob_{\cH_0}[T = 1|X,\tilde{X}] + \Prob_{\cH_1}[T = 0|X,\tilde{X}] \right\} \\
\geq 
	&\underset{(\theta^*, \bar\theta) \in \wh\Theta}{\sup} 
\left\{ \Prob_{\bar\cH_0} [T_{LR} = 1|X,\tilde{X}] + \Prob_{\bar\cH_1} [T_{LR} = 0|X,\tilde{X}] \right\}, 
%\\
%=
%	&\underset{(\theta_0, \theta_1) \in \wh\Theta(\Delta^2)}{\sup} 
%\left\{ \Prob_{\bar\cH_0} [T_{LR} = 1|X,\tilde{X}] + \Prob_{\bar\cH_1} [T_{LR} = 0|X,\tilde{X}] \right\},
\end{aligned}
\]
with~$T_{LR}$ being the test given by~\eqref{eq:test-oracle}. 
%here the last transition is due to~$\wh\Theta(\Delta^2)$ being permutation-invariant.
%where $T^{o}$ is given by $T^{o} := \ind\{  g_0(X,Y,\tilde{X},\tilde{Y}) \leq g_1(X,Y,\tilde{X},\tilde{Y}) \}$ and $g_0$ (resp. $g_1$) is the likelihood of $(Y,\tilde{Y})$ under $H_0$ (resp. under $H_1$) conditionally on $(X,\tilde{X})$.
Fixing~$(\theta^*, \bar\theta) \in \wh\Theta = \wh \Theta(32\Delta^2)$, under~$\bar \cH_0$ we get
\begin{align*}
&\Prob_{\bar\cH_0}[T_{LR} = 1|X,\tilde{X}] \\ 
%%%\Prob_0\left[T^* = 1|X,\tilde{X}\right] 
&\geq
\Prob \left\{ \| Y - X\theta_0\|^2 + \| \wt Y - \wt X \theta_1\|^2 \geq \| Y - X\theta_1\|^2 + \| \wt Y - \wt X \theta_0\|^2 \; \middle| \; X, \wt X \right\} \\
&= 
\Prob \left\{ 2\langle \xi,X(\theta_0-\theta_1) \rangle + 2\langle \tilde{\xi},\tilde{X}(\theta_0-\theta_1) \rangle \geq \|X(\theta_0 - \theta_1)\|^2 + \| \tilde{X}( \theta_0 - \theta_1)\|^2 \; \middle| \; X, \wt X  \right\} \\
&\geq 
C\exp\big(-c\max [\|X(\theta_0-\theta_1)\|^{2}, \|\wt X(\theta_0-\theta_1)\|^{2}]\big) 
=
C\exp\big(-cn\max[\wh \Delta_0^2,\wh\Delta_1^2]\big);
\end{align*}
here we first used that~$\langle \xi,X(\theta_0-\theta_1) \rangle \sim \cN(0,\|X(\theta_0-\theta_1)\|^2)$ and~$\langle \tilde{\xi},\tilde{X}(\theta_0-\theta_1) \rangle \sim \cN(0,\| \tilde{X}( \theta_0 - \theta_1)\|^2)$ conditionally to~$(X,\wt X)$, and then applied the lower bound for the Gaussian tails (see~\cite[Eq.~7.1.13]{stegun}):
\[
\Prob[\cN(0,1) \ge t] \ge Ce^{-t^2}, \quad \forall t \ge 0.
\]
%where we concluded using a lower  tail for the Gaussian cdf as in formula 7.1.13 in 
By symmetry, we also have the same bound for~$\Prob_{\bar\cH_1}[T_{LR} = 0|X,\tilde{X}]$. 
%Finally, the set~$\wh \Theta(\Delta^2)$ is permutation-invariant, hence taking constraint~$(\theta_0, \theta_1) \in \Theta(\Delta^2)$ Thus, the lower bound on
Now, taking~$(\theta_*, \bar\theta)$ on the boundary of~$\wh\Theta(32\Delta^2)$, i.e., such that~$\max[\wh \Delta_0^2, \wh \Delta_1^2] = 32\Delta^2$, we arrive at 
\begin{equation}\label{eq:lower-easy}
\underset{T: (\theta^*,X,Y,\wt X,\wt Y) \to \{0,1\}}{\inf} \;
	\underset{(\theta_0, \theta_1) \in \wt\Theta(\Delta^2)}{\sup} 
\left\{\Prob_{\cH_0}[T = 1|X,\tilde{X}] + \Prob_{\cH_1}[T = 0|X,\tilde{X}] \right\}\ge  C \exp (-c' n^{\vphantom 2} \Delta^2 ),
\end{equation}
which is the rank-independent part of~\eqref{eq:lower-fixed-design}.
Next we deal with the harder rank-dependent part.

\subsection{Rank-dependent bound}
\label{sec:lower-hard}
We first observe that in the cases~$n\Delta^2 \le 1$ and~$n\Delta^2 \ge \wh\rmin$, 
%with arbitrary chosen constants~$c', C' > 0$, 
the bound~\eqref{eq:lower-fixed-design} follows from~\eqref{eq:lower-easy} up to a change in constants. %and we are done. 
Hence, it suffices to focus on the range 
\begin{equation}
\label{eq:Delta-range-for-complex-lower}
1 \leq n\Delta^2 \leq {\wh\rmin}.
\end{equation} 
%for some $c_1>0$. 
%large enough. In particular this suggests that $\underbar{r}$ can be assumed to be large enough. Let $\Delta$ satisfy the previous conditions.
Instead of fixing the pair~$(\theta^*,\bar\theta)$, we now only fix~$\theta^*$ 
and put on~$\bar \theta$ a Gaussian prior centered at~$\theta^*$ with covariance corresponding to the constraint~$(\theta^*,\bar \theta) \in \wh\Theta$. Note that, by symmetry, this is the same as putting the same prior on~$(\theta_0, \theta_1)$, or the centered prior with the same covariance on~$\theta_1 - \theta_0$. 
Technically, such prior violates the constraint~$(\theta_0, \theta_1) \in \wh \Theta$, so we must verify that the event
\begin{equation}
\label{eq:constraint-set-event}
\cC := \{(\theta_0, \theta_1) \in \wh \Theta\}
\end{equation}
has sufficient mass under this prior. (Note that this {\em concentration step} is common in the literature on Bayesian lower bounds, see, e.g.,~\cite[Sec.~5.4]{johnstone2017gaussian}.)
To that end, we further proceed in three steps.

%\begin{itemize}
%\item 
\proofstep{1}: \textbf{{\em Reduction to the unconstrained Bayes risk.}}
We let $\pi$ be any prior on~$(\theta_0,\theta_1) \in \R^d$, and let~$\pi_{\cC}$ be the conditioning of~$\pi$ to the event~$\cC$ in~\eqref{eq:constraint-set-event}:
\[
\piC(\cE) = \frac{\pi (\mathcal{\cE} \cap \cC)}{\pi(\cC)}, \quad \forall \cE \subseteq \R^{2d}.
\]
In what follows, we identify events over~$(\theta_0, \theta_1)$ with subsets of~$\R^{2d}$; in particular,~$\cC$ is identified with~$\wh \Theta = \wh\Theta(32\Delta^2)$.
%and we write~$\wh \Theta = \wh \Theta(\Delta^2)$ for simplicity. 
%Finally, let~$(\theta_0,\theta_1)^{\cC} = (\theta_0,\theta_1) \cdot \ind_{\cC}$ for brevity. 
Now, since~$\pi_\cC$ is supported on~$\cC$, we can bound the left-hand side of~\eqref{eq:lower-fixed-design} as
\begin{equation*}
%\underbrace{
\underset{T}{\inf} 
\underset{(\theta_0,\theta_1) \in \wh\Theta}{\sup} \Prob_{\cH_0}[T = 1|X,\wt X] + \Prob_{\cH_1}[T = 0|X,\wt X]
%}_{L(A)}
\ge 
\underset{T}{\inf} \; \E_{\pi_\cC}\Big[ \Prob_{\cH_0}[T = 1|X,\wt X] + \Prob_{\cH_1}[T = 0|X,\wt X]\Big],
\end{equation*}
where $\E_{\pi_\cC}$ is the expectation over~$(\theta_0, \theta_1) \sim \pi_{\cC}$, and the infinum on the right is over the same set of admissible tests~$(\theta^*, X,Y,\wt X, \wt Y) \to \{0,1\}$ as on the left.
%According to~\cite[p.~228,~Corollary~1.2]{LC}, 
Now, let~$T_{\pi_{\cC}}$ be the corresponding Bayes test on which the Bayes risk is attained:
\[
\underset{T}{\inf} \; \E_{\pi_\cC}\Big[ \Prob_{\cH_0}[T = 1|X,\wt X] + \Prob_{\cH_1}[T = 0|X,\wt X]\Big] 
%= 
%\underset{T}{\inf} \; \E_{\pi_{\cC}} \left(\Prob_0[\wt T = 1|X,\tilde{X}] + \Prob_1[\wt T = 0|X,\tilde{X}]\right) 
= 
\E_{\pi_{\cC}} \left[\Prob_{\cH_0}[T_{\pi_{\cC}} = 1|X,\tilde{X}] + \Prob_{\cH_1}[T_{\pi_{\cC}} = 0|X,\tilde{X}] \right].
\]
On the other hand, 
\begin{align*}
%\underset{\wt T}{\inf} E_{\pi} \left(\Prob_0[\wt T = 1|X,\tilde{X}] + \Prob_1[\wt T = 0|X,\tilde{X}] \right)& \leq E_{\pi} \left(\Prob_0[\wt T^A = 1|X,\tilde{X}] + \Prob_1[\wt T^A = 0|X,\tilde{X}]\right)\\ \nonumber
\E_{\pi} \left[ \Prob_{\cH_0}[ T_{\pi_\cC} = 1|X,\tilde{X}] 
	+ \Prob_{\cH_1}[T_{\pi_\cC} = 0|X,\tilde{X}] \right]
&\le \E_{\pi_{\cC}} \left[ \Prob_{\cH_0}[ T_{\pi_\cC} = 1|X,\tilde{X}] 
	+ \Prob_{\cH_1}[  T_{\pi_\cC} = 0|X,\tilde{X}] \right] \\
&\quad + 2\pi(\R^{2d} \setminus \cC).
 \end{align*}
Finally, since~$T_{\pi_{\cC}}$ is generally not the Bayes test for~$\pi$, we have
\[
\underset{T}{\inf} \; \E_{\pi}\Big[ \Prob_{\cH_0}[T = 1|X,\wt X] + \Prob_{\cH_1}[T = 0|X,\wt X]\Big] 
\le 
\E_{\pi}\left[\Prob_{\cH_0}[T_{\pi_\cC}=1|X,\tilde{X}] 
	+ \Prob_{\cH_1}[T_{\pi_\cC}=0|X,\tilde{X}]\right].
\]
We conclude that
\begin{equation}
\label{eq:unconstrained}
\begin{aligned}
&\underset{T}{\inf} 
\underset{(\theta_0,\theta_1) \in \wh\Theta}{\sup} \Prob_{\cH_0}[T = 1|X,\wt X] + \Prob_{\cH_1}[T = 0|X,\wt X] \\
&\geq 
\underset{T}{\inf} \, \E_{\pi} \left[\Prob_{\cH_0}[T = 1|X,\tilde{X}] + \Prob_{\cH_1}[T = 0|X,\tilde{X}] \right] - 2\pi(\R^{2d} \setminus \cC);
\end{aligned}
\end{equation}
thus, it suffices to bound the Bayes risk associated with~$\pi$ from below and~$\pi(\R^{2d} \setminus \cC)$ from above.

%\item 
\proofstep{2}: \textbf{\em Choosing a prior and showing concentration.}
We choose~$\pi$ as follows:~$\theta^*$ is fixed at an arbitrary value, and
\begin{equation}
\label{eq:prior-definition}
\theta_1-\theta_0 \sim \mathcal{N}(0, \rho \wh \bSigma_0^\pinv) 
\;\; \text{with} \;\;
\rho :=  \frac{64\Delta^2}{\wh{r_0}}.
\end{equation}
%with the scaling factor~$ = \frac{2\sqrt{n}\Delta}{\sqrt{\wh r_0}}.$ 
Writing~$\cC = \wh\Theta(32\Delta^2)$, cf.~\eqref{def:set-empirical}, as~$\cC = \cC_0 \cup \cC_1$ with~$\cC_k = \{\wh \Delta_k^2 \geq 32\Delta^2\}$,~$k \in \{0,1\}$, and recalling that~$\wh \Delta_0^2 = \|\wh \bSigma_0^{1/2} (\theta_1 - \theta_0)\|^2 = \frac{1}{n}\|X (\theta_1 - \theta_0)\|^2$,  we see that 
\[
\pi(\R^{2d} \setminus \cC) 
\leq \pi(\R^{2d} \setminus \cC_0) 
= \pi ( \{ \wh \Delta_0^2 \leq 32 \Delta^2 \} ).
%= \pi ( \{ \| X(\theta_1-\theta_0)\|^2 \leq 32n\Delta^2 \} ).
\]
Clearly,
\begin{equation}
\label{eq:prior-prediction-residual}
\tfrac{1}{\sqrt{n}}X(\theta_1-\theta_0) \sim \mathcal{N}\left(0, \rho \bPi_X\right).
\end{equation}
Thus,~$\wh \Delta_0^2 \sim \rho \chi^2_{\wh r_0}$,~$\wh\Delta_0^2 / (32\Delta^2) \sim \tfrac{2}{\wh r_0} \chi^2_{\wh r_0},$ and, using the bound~\eqref{eq:tail-bounds-chi-sq-left} for the left tail of~$\chi^2$, we have
\[
\pi ( \R^{2d} \setminus \cC ) \leq \exp \left(-c \wh r_0 \right) \le \exp(-c\wh\rmin). 
\]
for some~$c > 0$.
Exchanging the roles of~$X$ and~$\wt X$, we see that the final bound is also valid for the counterpart~$\wt \pi$ of~$\pi$ based on~$\wt X$, i.e., such that~$\theta_1 - \theta_0 \sim \cN(0, \rho_1 \wh\bSigma_1^{\pinv})$ with~$\rho_1 = 64\Delta^2/\wh r_1$.
Now, recall that we work in the regime where~$n\Delta^2 \le \wh\rmin$, cf.~\eqref{eq:Delta-range-for-complex-lower}, and thus
\[
\exp(-c\wh\rmin) \le \exp\left(-\frac{cn^2\Delta^4}{\wh\rmin}\right).
\]
%The previous result holds also replacing $X^{\top}X$ by $\wt X^\top \wt X$. 
%Under the conditions we consider on $\Delta$, we have that $e^{-cn^2\Delta^{4}/\rmin}$ is much larger than $e^{-c\rmin}$. 
Recalling the result of~\proofstep{1} (namely~\eqref{eq:unconstrained}) we conclude that, in order to establish the~$\wh\rmin$-dependent part of~\eqref{eq:lower-fixed-design}, it suffices to lower-bound the {\em largest} of the two Bayes risks associated with~$\pi$ and~$\wt\pi$ as
\begin{align}
\underset{T}{\inf} \left\{ \E_{\pi} \left[\Prob_{\cH_0}[T = 1|X,\tilde{X}] + \Prob_{\cH_1}[T = 0|X,\tilde{X}] \right] \right\} 
&\vee 
\underset{T}{\inf} \left\{ \E_{\wt\pi} \left[\Prob_{\cH_0}[T = 1|X,\tilde{X}] + \Prob_{\cH_1}[T = 0|X,\tilde{X}] \right] \right\} \notag\\
&\geq 3\exp \left(-\frac{cn^2\Delta^{4}}{\wh\rmin}\right).
\label{eq:bayes-risk-alternative}
\end{align}
%for large enough~$C$ (e.g.,~$C = 3$ suffices). 

In the next step we prove~\eqref{eq:bayes-risk-alternative}; it is in this step that we use the fact that~$\wh\bSigma_0$ and~$\wh\bSigma_1$ commute.

\proofstep{3}: \textbf{\em Lower-bounding the Bayes risk.}
For~$\pi$ chosen in~\proofstep{2}, the Neyman-Pearson lemma gives
%\[
%\underset{\wt T}{\inf} E_{\pi}\left(\Prob_0[\wt T = 1|X,\tilde{X}] + \Prob_1[\wt T = 0|X,\tilde{X}]\right) \geq E_{\pi}\left(   \Prob_0\left[T^* = 1|X,\tilde{X}\right] + \Prob_1\left[T^* = 0|X,\tilde{X}\right]\right),
%\]
\[
\underset{T}{\inf} \E_{\pi} \left[\Prob_{\cH_0}[T = 1|X,\tilde{X}] + \Prob_{\cH_1}[T = 0|X,\tilde{X}] \right]  
\ge 
\E_{\pi} \left[\Prob_{\cH_0}[T_{MLR} = 1|X,\tilde{X}] + \Prob_{\cH_1}[T_{MLR} = 0|X,\tilde{X}] \right],
\]
where~$T_{MLR}$ is the {\em marginal likelihood ratio} test associated with~$\pi$ and given by
\[
T_{MLR} = \ind\{  Q_{\cH_0}(Y,\wt Y | X,\wt X) \leq Q_{\cH_1}(Y,\wt Y | X,\wt X)\},
\] 
where~$Q_{\cH_0}(Y,\wt Y | X,\wt X)$ (resp.,~$Q_{\cH_1}(Y,\wt Y | X,\wt X)$) is the marginal, over~$\bar \theta \sim \pi$, likelihood of~$(Y,\tilde{Y})$ under~$\cH_0$ (resp.,~$\cH_1$) conditionally on~$(X,\wt X)$.
Now, recalling that~$\cH_1$ reads~$(\theta^*, \bar\theta) = (\theta_1, \theta_0)$, we get
\[
Q_{\cH_1}^2(Y,\wt Y | X,\wt X) 
= \frac{
\exp\left(-\|\wt Y - \wt X\theta^{*}\|^2 - (Y- X\theta^*)^\top\left(\Id + n\rho\bPi_X\right)^{-1}(Y - X\theta^*) \right)
}{
C_n \det\left(\Id + n \rho \bPi_X\right)
},
\]
where~$C_n$ is the normalization constant depending solely on~$n$.
Indeed: conditionally on~$(X,\wt X)$, under~$\cH_1$ we have~$\wt Y \sim \cN(\wt X\theta^*,\Id)$,~$X\bar\theta \sim \cN(X\theta^*,n\rho \bPi_X)$
by~\eqref{eq:prior-prediction-residual}, and~$Y - X\bar\theta \sim \cN(0,\Id)$ independently; hence,~$Y \sim \cN(X\theta^*, \Id + n\rho \bPi_X)$ marginally over~$\bar\theta$.
%\[
%Q_{\cH_0}^2(Y,\wt Y | X,\wt X) = \frac{\exp\left(- \|Y - X\theta^{*}\|^2 - (\tilde{Y} - \tilde{X}\theta^*)^\top\left(\Id + \frac{4n\Delta^2}{\hat{r}_1}\bPi_X\right)^{-1}(\tilde{Y} - \tilde{X}\theta^*) \right)}{\left|\Id + \frac{4n\Delta^2}{\hat{r}_1}\bPi_X\right|},
%\]
Similarly,
\[
Q_{\cH_0}^2(Y,\wt Y | X,\wt X) 
= \frac{
\exp\left(-\|Y-X\theta^{*}\|^2-(\wt Y-\wt X\theta^*)^\top(\Id + n\rho\bOmega_{X,\wt X})^{-1}(\wt Y - \wt X \theta^*) \right)
}{
C_n \det (\Id + n \rho \bOmega_{X,\wt X})
},
\]
where~$\bOmega_{X,\wt X} := \wt X (X^\top X)^{\pinv}\wt{X}^\top$.
%\[
%Q_{\cH_1}^2(Y,\wt Y | X,\wt X) = \frac{\exp\left(- \|\tilde{Y} - \tilde{X}\theta^{*}\|^2 - (Y - X\theta^*)^\top\left(I + \frac{4n\Delta^2}{\hat{r}_1}\tilde{X}(X^\top X)^+\tilde{X}^\top\right)^{-1}(Y - X\theta^*) \right)}{\left|I + \frac{4n\Delta^2}{\hat{r}_1}\tilde{X}(X^\top X)^+\tilde{X}^\top\right|},
%\]
Hence,~$T_{MLR}$ writes
\[
T_{MLR} = \ind\{  \|\bA^{1/2}(Y- X\theta^*)\|^2 - \log\det(\Id-\bA) 
\geq \|\bB^{1/2}(\wt Y- \wt X\theta^*)\|^2 - \log\det(\Id-\bB)\},
\]
where 
\[
\bA := \Id - (\Id + n\rho\bPi_X)^{-1} 
\quad \text{and} \quad 
\bB := \Id - (\Id + n\rho\bOmega_{X,\wt X})^{-1}.
\]
%\[
%J_1 = I - \left(I + \frac{4n\Delta^2}{\hat{r}_1}\tilde{X}(X^\top X)^+\tilde{X}^\top\right)^{-1} \quad \text{and} \quad J_2 = I - \left(I + \frac{4n\Delta^2}{\hat{r}_1}\bPi_X\right)^{-1}.
%\]
Let us now lower-bound the marginal over~$\pi$ type I error~$\E_{\pi} \Prob_{\cH_0}[T_{MLR} = 1|X,\wt X]$. (Clearly this also gives a lower bound for the expected sum of errors.)
To this end, observe that
\[
\bA = \frac{n\rho}{1+ n\rho} \bPi_X,
\] 
and, under~$\cH_0$ and conditionally on~$(X,\wt X)$, we have
\[
\|\bA^{1/2}(Y- X\theta^*)\|^2 \sim \frac{n\rho}{1+n\rho}\|\bPi_X \xi\|^2  \quad \text{and} \quad \|\bB^{1/2}(\wt Y- \wt X\theta^*)\|^2 \sim n\rho \| \bOmega_{X,\wt X}^{1/2} \zeta \|^2,
\]
%\[
%\| \tilde{Y}-\tilde{X}\theta^* \|_{J_2}^2 \sim \frac{4n\Delta^2/\hat{r}_1}{1+ 4n\Delta^2/\hat{r}_1}\|\tilde{\xi}\|^2  \quad \text{and} \quad \| Y-X\theta^* \|_{J_1}^2 \sim \sum_{i=1}^{\hat{r}_1}\mu_i\xi_i^2,
%\]
where~$\xi [= Y-X\theta_0] \sim \cN(0,\Id)$, and~$\zeta$ is independent from~$\xi$ and has the same distribution ($\zeta$ is the whitening of~$\wt Y - \wt X\theta_0 = \wt \xi + \wt X(\theta_1 - \theta_0)$). 
By rotation invariance, we may w.l.o.g.~assume that
%~$\bPi_X = \sum_{j=1}^{\wh r_0} \ue_j \ue_j^\top$, where~$\ue_j$ is the~$j$-th canonical basis vector of~$\R^n$. Similarly, we may w.l.o.g. assume that
\[
n\rho \bOmega_{X,\wt X} = \sum_{j=1}^{\wh r_0} \mu_j \ue_j \ue_j^\top,
\]
where~$\ue_j$ is the~$j$-th canonical vector of~$\R^n$; here we used that~$\rank(\bOmega_{X,\wt X}) \le \wh r_0$ (in fact,~$\rank(\Omega_{X,\wt X})$ is precisely~$\min[\wh r_0, \wh r_1]$ if~$\wh \bSigma_0,\wh \bSigma_1$ commute.) 
Thus, 
\[
\E_\pi\Prob_{\cH_0}\left[T_{MLR} = 1|X,\tilde{X}\right] 
=
\Prob\left[ 
\|\bPi_X{\xi}\|^2 
\geq 
\frac{1+ n\rho}{n\rho}\left(\wh r_0 \log(1+n\rho) + \sum_{j=1}^{\wh r_0} \mu_j\zeta_j^2 - \log(1+\mu_j) \right) \right].
\]
Now, by the standard deviation bound the generalized chi-squared distribution (\cite[Lemma~1]{laurent2000adaptive}), 
\[
\sum_{j=1}^{\hat{r}_0} \mu_j\zeta_j^2 \leq \sum_{j=1}^{\wh r_0} \mu_j + 2\sqrt{\sum_{j=1}^{\wh r_0}\mu_j^2}
\] 
with probability~$c > 0$. 
Moreover,~$\mu_j - \log(1+\mu_j) \leq \mu_j^2$. Hence
\[
\E_\pi \Prob_{\cH_0}\left[T_{MLR} = 1|X,\tilde{X}\right] 
\geq 
c\Prob\left[ \|\bPi_{X} \xi\|^2 \geq \frac{1+n\rho}{n\rho} \left( \hat{r}_0\log(1+n\rho) + \sum_{j=1}^{\hat{r}_0} \mu_j^2 + 2\sqrt{\sum_{j=1}^{\hat{r}_0}\mu_j^2}\right) \right].
\]
Moreover,~$\log(1+n\rho) - \frac{n\rho}{1+n\rho} \leq (n\rho)^2$ and~$n\rho \le 1$ (cf.~\eqref{eq:Delta-range-for-complex-lower}), so we arrive at
\begin{equation}
\label{eq:before-commutativity-argument}
\E_\pi\Prob_{\cH_0}\left[T_{MLR} = 1|X,\tilde{X}\right] 
\geq 
c\Prob\left[ \|\bPi_{X} \xi\|^2   - \hat{r}_0 \geq \frac{2}{n\rho}\left( \sum_{j=1}^{\hat{r}_0}\mu_j^2+2\sqrt{\sum_{j=1}^{\hat{r}_0}\mu_j^2}\right) + 2 \wh r_0 n\rho \right].
\end{equation}
Now, observe that we can w.l.o.g. assume that~$\|\bOmega_{X,\wt X}\| \le 1$ in operator norm. Indeed, recall that, by our assumption,~$\wh \bSigma_0 = \tfrac{1}{n} X^\top X$ and~$\wh \bSigma_1 = \tfrac{1}{n} \wt X^\top \wt X$ commute, and hence are diagonalized in the same orthonormal basis; w.l.o.g., we can assume this basis to be~$\ue_1, ..., \ue_{\wh r_0}$. 
One can then verify that the (non-zero) eigenvalues of~$\bOmega_{X,\wt X} = \wt X (X^\top X)^{\pinv}\wt{X}^\top$  are~$\alpha_j/\beta_j$, where~$\alpha_j$ (resp.~$\beta_j$) is the eigenvalue of~$\wh \bSigma_0$ (resp.,~$\wh \bSigma_1$) corresponding to~$\ue_j$. On the other hand, the eigenvalues of~$\bOmega_{\wt X, X} = X (\wt X^\top \wt X)^{\pinv} X^\top$ are~$\beta_j/\alpha_j$. %, the inverses of those of~$\bOmega_{X,\wt X}$. 
Hence, at least half of the eigenvalues for~$\bOmega_{X,\wt X}$ or~$\bOmega_{\wt X, X}$ are at most~$1/2$, and we can w.l.o.g.~assume that this is the case for~$\bOmega_{X,\wt X}$, since otherwise we can simply exchange the roles of~$X$ and~$\wt X$ as explained in step~\proofstep{2}. (Note that this will also change~$\wh r_0$ in the present argument to~$\wh r_1$, and this is why in~\eqref{eq:lower-fixed-design} we have~$\wh\rmin = \min[\wh r_0, \wh r_1]$, i.e., the worst case.) Finally, for the remaining eigenvalues we can simply avoid the corresponding eigenvectors to begin with, when constructing the prior~$\pi$ in step~\proofstep{2}. More precisely, one can easily verify that the boung~$\pi(\R^{2d} \setminus \cC) \le \exp(-c\wh r_0)$ proved in step~\proofstep{2} remains valid for~$\pi$ adjusted in this way, with~$c$ becoming~$c/2$; similarly one can routinely adjust the subsequent analysis in step~\proofstep{3}. To summarize, we can safely assume that~$\|\bOmega_{X,\wt X}\| \le 1$, and thus~$\mu_j \le n\rho$ for all~$j$. Returning to~\eqref{eq:before-commutativity-argument}, and recalling the definition of~$\rho$ (cf.~\eqref{eq:prior-definition}), this leads to
\[
\begin{aligned}
\E_\pi\Prob_{\cH_0}\left[T_{MLR} = 1|X,\tilde{X}\right] 
&\geq 
c\Prob\left[ \|\bPi_{X} \xi\|^2-\hat{r}_0 \geq 4\sqrt{\wh r_0}+4\wh r_0 n\rho \right] \\
&=
c\Prob\left[ \|\bPi_{X} \xi\|^2-\hat{r}_0 \geq 4\sqrt{\wh r_0}+256 n \Delta^2 \right].
\end{aligned}
\]
%
%Assuming that for all~$i$ we have~$\mu_i \leq 4n\Delta^2/\hat{r}_1$ (or equivalently~$\|\tilde{X}(X^\top X)^+\tilde{X}^\top \|_{\infty} \leq 1$)\footnotemark \footnotetext{This condition in particular holds w.l.o.g if~$X^{\top}X$ and~$\tilde{X}^{\top}\tilde{X}$ commute. Indeed, in this case both matrices are diagonalized in the same orthonormal basis. Exchanging the roles of $X$ and $\tilde{X}$, we can always assume that the number of eigenvalues~$\lambda_i(\tilde{X}(X^\top X)^+\tilde{X}^\top)$ smaller than~$1$ is larger than~$\underbar{r}/2$. Hence we can replace~$(X^{\top}X)^{+}$, in the choice of~$\pi$, with the submatrix of rank at least~$\underbar{r}/2$ corresponding to the small eigenvalues~$\lambda_i(\tilde{X}(X^\top X)^+\tilde{X}^\top)$.}, we get moreover that 
%\[
%2E_\pi\Prob_1\left[T^* = 0|X,\tilde{X}\right] \geq \Prob\left[ \|\tilde{\xi}\|^2 - \hat{r}_1 \geq 4\sqrt{\hat{r}_1} + 16n\Delta^2\right].
%\]
We are now in the position to apply a lower bound for the right tail of~$\chi^2_k$ distribution with~$k \ge 2$ degrees of freedom (\cite[Prop.3.1]{inglot}):\footnotemark
\begin{equation*}
%\label{eq:tail_square}
\Prob \left[ \chi_k^2 - k \geq u \right] \geq \frac{c(u+k)}{\sqrt{k}(u+\sqrt{k})} \exp \left(-\frac{Cu^2}{k}\right),
\end{equation*}
This bound, when applied with~$k = \wh r_0$ and~$u = 4\sqrt{\wh r_0} + 256 n\Delta^2$,  suffices for our purposes. 
Indeed, recall that we are in the regime~$n \rho \le 1$, i.e.,~$n\Delta^2 = O(\wh r_0)$. Thus, we need to apply the bound in the range~$c_1 \sqrt{k} \le u \le c_2 k$, where it becomes
\begin{equation}
\label{eq:chi-squared-lower-estimates}
\begin{aligned}
\Prob \left[ \chi_k^2 - k \geq u \right] \geq 
\frac{c\sqrt{k}}{u} \exp \left(-\frac{Cu^2}{k}\right) 
\ge c\exp \left(-\frac{2Cu^2}{k}\right) 
&\ge c\exp \left(-\frac{C'(\sqrt{\wh r_0} + n\Delta^2)^2}{\wh r_0}\right) \\
&\ge c' \exp \left(-\frac{C'' n^2 \Delta^4}{\wh r_0}\right).
\end{aligned}
\end{equation}
This proves the~$\wh \rmin$-dependent part of~\eqref{eq:lower-fixed-design}. 
Next we exhibit design distributions~$\cD_0$,~$\cD_1$ satisfying the requirements in Sec.~\ref{sec:lower-fixed-design-reduction}; recalling the discussion in Sec.~\ref{sec:lower-fixed-design-reduction}, this concludes the proof of the theorem.  

\footnotetext{One can verify that this bound is tight (matching~\eqref{eq:tail-bounds-chi-sq-right}) when~$u = O(k)$, which is our case; however, it is loose for larger deviations.
The recent work~\cite[Corollary~3]{zhang2018non} verifies the sharpness of~\eqref{eq:tail-bounds} in all regimes.}

\subsection{Constructing~$\cD_0, \cD_1$ with commuting~$\wh \bSigma_0, \wh \bSigma_1$}
\label{sec:lower-orths}

%Here we construct distributions~$\cD_0, \cD_1$ that satisfy the requirements in Sec.~\ref{sec:lower-fixed-design-reduction}.
%for the design~$X, \wt X$ such that~$X^\top X$ and~$\wt X^\top \wt X$ commute, and other requirements in the previous argument also hold with high probability. 
Let us fix some~$r \le d$ and generate the rows of~$X$ as follows:
\[
x_i \sim \sqrt{r} \sigma_i \ue_{k_i}, \quad i \in [n],
\]
where~$\ue_k$ is the~$k$-th canonical vector in~$\R^d$, each~$k_i$ is sampled uniformly on~$[r]$ i.i.d.~over~$i \in [n]$, and~$(\sigma_i)$ is the i.i.d.~sequence of Rademacher random variables independent from~$(k_i)$. In other words, we sample uniformly from~$\{\pm \ue_1, ..., \pm \ue_r\}$. Similarly, the rows of~$\wt X$ are
$
\wt x_i \sim \sqrt{r_1} \wt\sigma_i \ue_{\wt k_i}, \; i \in [n],
$
independently of~$X$, with~$\wt k_i \sim \text{Uniform}([r_1])$. 
One can easily verify that the covariance of~$x_i$ is
\[
\bSigma := \E[\tfrac{1}{n}X^\top X] = \bPi_{r},
\]
the projector on the span of~$\ue_1, ..., \ue_r$; in particular,~$\rank(\bSigma_0) = r$. Similarly,~$\bSigma_1 = \E[\tfrac{1}{n}\wt X^\top \wt X] = \bPi_{r_1}$; w.l.o.g.~we now focus on~$X$.
Now, the sample covariance is
\begin{equation}
\label{eq:covariance-orthonormal}
\wh \bSigma := \frac{r}{n} \sum_{i=1}^n \ue_{k_i} \ue_{k_i}^\top,
\end{equation}
and~$\wh\bSigma$ has a similar form;
clearly,~$\wh \bSigma$ and~$\wh \bSigma_1$ commute.
Moreover,~$\wh r := \rank(\wh \bSigma) \le \min[r,n]$~a.s., and this bound is essentially sharp up to a constant factor. More precisely, we have the following result.

\begin{lemma}
One has~$\E[\wh r] \ge \min[r,n]/2$. Moreover,~$\wh r \ge \min[r,n]/4$ with probability at least~$1/8$.
%\[
%\begin{aligned}
%\Prob[\wh r < r] &\le \exp\left(-\frac{n}{2r}\right) \; \text{when} \; n \ge 2r \ln r, \\
%\Prob[\wh r < n/2] &\le \exp\left(-n/8\right) \; \text{when} \; 32 \le n \le r.
% \end{aligned}
%\]
\end{lemma}

\begin{proof}
Note that~$\wh r$ is the number of different terms in the sum~\eqref{eq:covariance-orthonormal}, so that~$\wh \bSigma = \sum_{k \in [r]} \nu_k$, where
\[
\nu_k := \ind\{\exists i \in [n]: k_i = k\}.
\]
Thus,~$\E[\wh r] = r P_{r,n}$, where~$P_{r,n} := \Prob[\nu_1 = 1]$ is given by
\[
P_{r,n} = 1-\left(1-\frac{1}{r}\right)^n
\] 
When~$n \ge r$, we have
\[
P_{r,n} \ge 1-\left(1-\frac{1}{r}\right)^r \ge 1-\frac{1}{e} > \frac{1}{2},
\]
and thus~$\E[\wh r] \ge r/2$. On the other hand, when~$n < r$, we have
\[
P_{r,n} = 1- \left(\left(1-\frac{1}{r} \right)^{r}\right)^{n/r}  \ge 1-e^{-n/r} \ge \frac{n}{r} - \frac{n^2}{2r^2} \ge \frac{n}{2r}
\]
where we used that~$e^{-t} \le 1 - t + t^2/2$ for~$0 \le t \le 1$. Thus,~$\E[\wh r] \ge n/2$  in this case. 
For the bound in probability, we can estimate the second moment~$\E[\wh r]$ and use the Paley-Zygmund inequality (\cite{paley1932note}):
\begin{equation}
\label{eq:paley-zygmund-for-rank}
\Prob\left\{ \wh r > t \E[\wh r] \right\} \ge (1-t)^2\frac{\E[\wh r]^2}{\E[\wh r^2]}.
\end{equation}
Assuming~$r \ge 2$ w.l.o.g., we have
\[
\begin{aligned}
\E[\wh r^2] = \E\left[\sum_{k,l \in [r]} \nu_k \nu_l\right] = \E[\wh r] + \E\left[\sum_{k \ne l \in [r]} \nu_k \nu_l \right] 
&= \E[\wh r] + r(r-1) \E[\nu_1 \nu_2] \\
&= r(r-1)\Prob\{\nu_1 = 1 \, \cap \, \nu_2 = 1\}.
\end{aligned}
\]
Moreover,
$
\Prob\{\nu_1 = 1 \, \cap \, \nu_2 = 1\} = 1-\Prob\{\nu_1 = 0 \, \cup \, \nu_2 = 0\}
$
and 
\[
\begin{aligned}
\Prob\{\nu_1 = 0 \, \cup \, \nu_2 = 0\} 
&= \Prob\{(\nu_1,\nu_2) = (0,0)\} + 2\Prob\{(\nu_1,\nu_2) = (0,1)\} \\
&= \left(1-\frac{2}{r}\right)^n + 2\left[\left(1-\frac{1}{r}\right)^n -  \left(1-\frac{2}{r}\right)^n\right],
%= 2\left(1-\frac{1}{r}\right)^n -  \left(1-\frac{2}{r}\right)^n,
\end{aligned}
\]
whence %, using that~$(1-1/x)^x \le 1/e \le (1-1/x)^{x-1}$ for all~$x > 1,$ 
we get
\[
\begin{aligned}
\Prob\{\nu_1 = 1 \, \cap \, \nu_2 = 1\} 
= 1-2\left(1-\frac{1}{r}\right)^n + \left(1-\frac{2}{r}\right)^n 
&\le \left[1-\left(1-\frac{1}{r}\right)^n \right]^2 
= P_{r,n}^2,
%&= (1-e^{-n/r})^2 
\end{aligned}
\]
and estimate
\[
\E[\wh r^2] \le \E[\wh r] + r(r-1) P_{n,r}^2 \le \E[\wh r] + \E[\wh r]^2 \le 2\E[\wh r]^2.
\]
Here in the end we used that~$\E[\wh r] \ge 1$ since~$\wh r \ge 1$ a.s. 
The result follows from~\eqref{eq:paley-zygmund-for-rank} with~$t=1/2$.
\end{proof}
%\proofstep{2}. We now show the bounds in probability. For the first bound, observe that
%\[
%\begin{aligned}
%\Prob[\wh r < r] 
%= \Prob\left[\sum \nu_k \le r-1 \right] %_{k \in [r]}
%= \Prob\left[\sum (1-\nu_k) \ge 1\right] 
%= \Prob\left[\sum \bar\nu_k \ge 1\right]
%\le r \Prob\left[\bar\nu_1 = 1\right] 
%= r (1-P_{r,n}),
%\end{aligned}
%\]
%where~$\bar\nu_k = (1-\nu_k)$ is defined as~$\nu_k := \ind\{k_i \ne k, \; \forall i \in [n]\}$, and we took the union bound. 
%Thus,
%\[
%\Prob[\wh r < r]  \le r\left(1-\frac{1}{r}\right)^n \le r e^{-n/r}. 
%\]
%Now, observe that~$n \ge 2r\ln r$ implies that~$r e^{-n/(2r)} \le 1$ and thus~$\Prob[\wh r < r] \le e^{-n/(2r)}$ as claimed.

%%%%%%%%%%%%%%%%%%%%%%%%%%%%%%%%%%%%%%%%%%%%%%%%%%%%%%%%%%%%%%%%%%%%%%%%%%%%%%%%%%%%%%%%%%%%

%It remains to verify that~$c\Delta^2 \le \wh \Delta^2 \le C\Delta^2$ with a fixed probability for some constants~$c,C$. Fixing~$z = \theta_1-\theta_0$, it suffices to bound~$\wh \Delta_0^2 = \|\wh \Sigma^{1/2} z\|^2$ by its expectation~$\Delta_0^2 \|\Pi_r z \|^2$ up to constants. The upper bound follows from Markov's inequality as~$\wh\Delta_0^2$ is non-negative. On the other hand, %For the lower bound, observe that %To this end, 
%\[
%\|\wh \Sigma^{1/2} z\|^2 = \frac{r}{n} \sum_{i = 1}^n z_{k_i}^2, 
%\]
%whence

%%%%%%%%%%%%%%%%%%%%%%%%%%%%%%%%%%%%%%%%%%%%%%%%%%%%%%%%%%%%%%%%%%%%%%%%%%%%%%%%%%%%%%%%%%%%

%\section{Upper bounds for non-linear models}

\section{Proof of Theorem \ref{th:asymptotic}}
\label{app:upper-general}
As in the proof of Theorem~\ref{th:upper-random-design}, we decompose the statistic whose sign is examined in~\eqref{eq:test-asymp} as~$\wh S = \wh S_0 - \wh S_1$. 
W.l.o.g., we analyze the type II error probability~$\Prob_{\cH_1}[\wh T = 0];$ thus,~$\theta^* = \theta_1$. 

\proofstep{1}.
Recall that~$\Mopt_1 := \M_1(\theta_1)$. 
We first study
\[
\begin{aligned}
\wh S_1 := n_1 \| \wh \H_1(\theta_1)^{\dagger/2} \nabla \wh L_1(\theta_1) \|^2 - \Tr(\Mopt_1)
% \wh S_0(\theta_0) = n_1 \| \wh \H_1^{-1/2}(\theta_0) \nabla \wh L_0(\theta_0) \|^2 - \Tr(\M_0(\theta_0)).
\end{aligned}
\]
and the complementary to it term within~$\wh S_0$. 
%  as~$n_1 \to \infty$.
Let us first define random variables
\[
Z(\theta) := \nabla \wh L_0(\theta) - \nabla L_0(\theta), \quad
\wt Z(\theta) := \nabla \wh L_1(\theta) - \nabla L_1(\theta);
\]
% which are centered under~$H_0$ and~$H_1$ correspondingly.
note also that~$\nabla L_0(\theta_0) = \nabla L_1(\theta_1) = 0$.
By the central limit theorem (CLT) we have the following convergence in distribution as~$n_0, n_1 \to \infty$: 
\[
\sqrt{n_0} Z(\theta) % \nabla \wh L_0(\theta_0) 
\weakto \cN(0,\G_0(\theta)), \quad 
\sqrt{n_1} \wt Z(\theta) % \nabla \wh L_1(\theta_1) 
\weakto \cN(0,\G_1(\theta)),
\]
with~$\G_0(\theta),\G_1(\theta)$ defined in~\eqref{eq:matrices-population}.
Define~$\chi^2_{\M}$ as the generalized chi-square law -- precisely, the law of~$\|\xi\|^2$ with~$\xi \sim \cN(0,\M)$ for PSD matrix~$\M$.
Recall that~$\E[\chi^2_{\M}] = \Tr[\M]$, and~\cite[Lemma~1]{laurent2000adaptive} gives
%we have
\begin{subequations}
\label{eq:generalized-chi-square}
\begin{align}
\label{eq:generalized-chi-square-right}
\Prob[\chi^2_{\M} - \Tr[\M] \ge t] &\le\exp \left(-c\min\left[\frac{t}{\|\M\|},\frac{t^2}{\Tr[\M^2]}\right]\right),\\
% \le \exp \left(-\frac{c}{\|\M\|}\min\left[t, \frac{t^2}{\Tr(\M)} \right]\right), \\
\label{eq:generalized-chi-square-left}
\Prob[\chi^2_{\M} - \Tr[\M] \le -t] &\le\exp \left(-\frac{ct^2}{\Tr[\M^2]}\right).
% \le \exp \left(-\frac{ct^2}{\|\M\|\Tr(\M)}\right)
\end{align}
\end{subequations}
At fixed~$\theta$ we have~$n_0 \| \H_0(\theta)^{\dagger/2} Z(\theta) \|^2 \weakto \chi^2_{\M_0(\theta)}$ and~$n_1 \| \H_1(\theta)^{\dagger/2} \wt Z(\theta) \|^2 \weakto \chi^2_{\M_1(\theta)},$ that is,
\[
n_1 \| \H_1(\theta_1)^{\dagger/2} \nabla \wh L_1(\theta_1) \|^2 \weakto \chi^2_{\Mopt_1}.
\]
since~$\nabla L_{\theta_1}(\theta_1) = 0$.
Clearly, the fully empirical counterpart of this quantity~$n_1 \| \wh \H_1(\theta_1)^{\dagger/2} \nabla \wh L_1(\theta_1) \|^2$ has
the same asymptotic distribution. 
Indeed, at any fixed~$\theta$ one has~$\wh \H_k(\theta) \to \H_k(\theta)$ in probability as~$n_k \to \infty$ by the law of large numbers; in particular,~$\wh \H_1(\theta_1) \to \H_1(\theta_1)$. 
Thus, by the matrix version of Slutsky's theorem~(\cite{van2000asymptotic}), we have that~$\wh\H_1(\theta_1)^{\dagger/2} \nabla \wh L_1(\theta_1) \weakto \cN(0, \Mopt_1)$, whence, indeed,
\[
n_1 \| \wh \H_1(\theta_1)^{\dagger/2} \nabla \wh L_1(\theta_1) \|^2 \weakto \chi^2_{\Mopt_1}.
\]
Using tail bounds~\eqref{eq:generalized-chi-square-right}--\eqref{eq:generalized-chi-square-left}, for any fixed~$t > 0$  we have
$
\Prob [\wh S_1 \ge t] 
\to 
% \Prob \big[ n_1 \| \H_1(\theta)^{-1/2} \nabla \wh L_1(\theta_1) \|^2_2 - \Tr[\M_1^*] \ge t \big] 
\Prob[\chi^2_{\Mopt_1} - \Tr[\Mopt_1] \ge t]
$
as~$n_1 \to \infty$. 
Now, recall that we are in the regime~$n_0 \to \infty$,~$\bar\Delta_0 \to 0$ with~$n_0\bar\Delta_0^2 \to \lambda_0 > 0$. 
Thus, choosing~$t = \lambda_0/3,$ and applying~\eqref{eq:generalized-chi-square-right}, we arrive at 
% and estimating~$\Tr(\M^2) \le \|\M\| \Tr(\M)$ for any~$\M \succcurlyeq 0$
\begin{equation}
\label{eq:limit-1}
\lim_{n_0, n_1 \to \infty} \Prob \left[ \wh S_1 \ge \frac{n_0\bar\Delta_0^2}{3} \right] \le 
\exp\left(-{c \lambda_0} \min \left[ \frac{1}{\|\Mopt_1\|}, \frac{\lambda_0}{\Tr[(\Mopt_1)^2]} \right] \right),
\end{equation}
where~$n_0, n_1 \to \infty$ as specified in the premise of the theorem, i.e., with~$n_0 \bar\Delta_0^2 \to \lambda_0$ and~$n_1 \bar\Delta_1^2 \to \lambda_1$.

\proofstep{2}.
We now consider~$\wh S_0$ which we decompose as 
% Since~$\wh \H_0(\theta_1) \to \H_0(\theta_1)$ a.s., we have
\[
\begin{aligned}
\wh S_0 
&:= n_0 \|\wh\H_0(\theta_1)^{\dagger/2} \nabla \wh L_0(\theta_1) \|^2 - \Tr[\M_0(\theta_1)] \\
&=
n_0 \| \wh\H_0(\theta_1)^{\dagger/2} Z(\theta_1) \|^2 -\Tr[\M_0(\theta_1)]  + n_0\bar\Delta_0^2 
%\\ & \hspace{5cm} 
+ 2 n_0 \langle \wh\H_0(\theta_1)^{\dagger/2} Z(\theta_1), \wh\H_0(\theta_1)^{\dagger/2} \nabla L_0(\theta_1) \rangle.
\end{aligned}
\]
% Moreover,
% \[
% n_0 \| \H_0(\theta_1)^{-1/2} \nabla \wh L_0(\theta_1) \|^2 = \]
We have~$n_0 \| \wh\H_0(\theta_1)^{\dagger/2} Z(\theta_1) \|^2 - \Tr[\M_0(\theta_1)] \weakto \chi^2_{\M_0(\theta_1)}$ by CLT combined with Slutsky's theorem (cf.~\proofstep{1}). Hence, using~\eqref{eq:generalized-chi-square-left}, we have
\begin{equation}
\label{eq:limit-2}
\begin{aligned}
\lim_{n_0, n_1 \to \infty}
\Prob \left[n_0 \| \wh\H_0(\theta_1)^{\dagger/2} Z(\theta_1) \|^2 - \Tr[\M_0(\theta_1)] \le - \frac{n_0\bar\Delta_0^2}{3}\right] 
&\le \exp\left(-\frac{c \lambda_0^2}{\Tr[\M_0^2(\theta_1)]} \right).
% \\ 
% &\to \exp\big(-\frac{c \lambda_0^2}{\Tr[\bar\M_0^2]} \big),
\end{aligned}
\end{equation}
%where the limit is in the same regime as before. 
% and the last transition is due to~$\bar\Delta_0 \to 0$. 
Now, by CLT combined with Slutsky's theorem,~$\sqrt{n_0} \wh\H_0(\theta_1)^{\dagger/2} Z(\theta_1) \weakto \cN(0,\M_0(\theta_1))$.
Due to that, and since~$\|\wh\H_0(\theta_1)^{\dagger/2} \nabla L_0(\theta_1)\|/ \bar\Delta_0 \to 1$ in probability, we have that
\[
\sqrt{n_0} \langle \wh\H_0(\theta_1)^{\dagger/2} Z(\theta_1), \wh\H_0(\theta_1)^{\dagger/2} \nabla L_0(\theta_1) \rangle \weakto \cN(0,v_0), \quad v_0 \le \|\M_0(\theta_1)\|\bar\Delta_0^2.
\]
Therefore by~\eqref{eq:tail-bounds-normal}, 
\begin{equation}
\label{eq:limit-3}
\lim_{n_0, n_1 \to \infty} 
	\Prob\left[ 2n_0 \langle \wh\H_0(\theta_1)^{\dagger/2} Z(\theta_1), \wh\H_0(\theta_1)^{\dagger/2} \nabla L_0(\theta_1) \rangle 
\le - \frac{n_0\bar\Delta_0^2}{3} \right] 
=\exp\left(\frac{-\lambda_0}{36\|\M_0(\theta_1)\|}\right).
\end{equation}
% Combining the previous results through the union bound, this gives
% \[
% \Prob \left[ \wh S_0(\theta_1) \ge \frac{2n_0\Delta_0^2}{3} \right] = 
% (2+o(1)) \exp\left(-\frac{c n_0 \Delta_0^2}{\|\M_0(\theta_1)\|} \min \left[ 1, \frac{n_0 \Delta_0^2}{\Tr(\M_0(\theta_1))} \right] \right).
% \]
Finally, combining~\eqref{eq:limit-1}--\eqref{eq:limit-3} through the union bound, and observing that~$\Tr[\M_0(\theta_1)] / \Tr[\Mopt_0] \to 1$ and~$\|\M_0(\theta_1) \| / \|\Mopt_0\| \to 1$ since~$\M_0(\cdot)$ is continuous at~$\theta_0$ and~$\bar\Delta_0 \to 0$, we arrive at the required bound %for the type II error probability:
\begin{equation}
\lim_{n_1,n_2 \to \infty} \Prob_{\cH_1}[\wh T = 0] 
\le 
C \exp\bigg(-c\lambda_0 \min \bigg[\frac{1}{\|\Mopt_0\|}, \; \frac{1}{\|\Mopt_1\|}, \; \frac{\lambda_0}{\Tr[(\Mopt_0)^2]}, \; \frac{\lambda_0}{\Tr[(\Mopt_1)^2]}\bigg]\bigg).
\end{equation}
(As before, the limit is in the regime~$n_k^{\vphantom 2} \bar\Delta_k^2 \to \lambda_k^{\vphantom 2}$.)
The type I error bound follows by symmetry.
\qed

\section{Proof of Theorem~\ref{th:glm-fixed-prob}}
%\underline{\bf Erratum.} 
%We admitted several inaccuracies in the formulation of Theorem~\ref{th:glm-fixed-prob} in the main text. First, the constants are larger. Second, the factors~$\kappa_0 - \nu_0^2,\kappa_1 - \nu_1^2$ in the lower bound for the sample size must be replaced with~$\kappa_0$ and~$\kappa_1$. Third, ~$\Var[\wh \Delta_1^2]$ must be replaced with the larger quantity~$\E[\wh \Delta_1^4]$. Finally, the probability of error is bounded by~$0.4$ rather than~$0.25$. 
%These changes must be propagated further on until the end of Section~\ref{sec:glm}. Below we give the corrected formulation of the theorem. 
% As in the proof of Theorem~\ref{th:asymptotic}, 
W.l.o.g.~we analyze the type II error~$\Prob_{\cH_1}[\wh T = 0]$, so that~$\theta^* = \theta_1$. 
For brevity, let
\[
\wh\Delta^2 := \wh\Delta^2_0, \quad 
\Delta^2 := \Delta_0^2, \quad 
a := a_0, \quad 
\nu := \nu_0, \quad 
\kappa := \kappa_0.
\]
% \eta_i := \eta_{x_i}.$
We first focus on the ``shifted'' term in~\eqref{eq:test-glm},
\[
\wh S_0 := \sum_{i=1}^{n} \frac{(a'(\eta_{i}(\theta_1)) - y_i)^2}{a''(\eta_{i}(\theta_1))} - n \nu(\theta_1),
\]
where~$\eta_i(\theta) := \eta_{x_i}(\theta)$ for brevity, and the data~$(x_1, y_1), ..., (x_n,y_n)$ are sampled from the distribution corresponding to the wrong hypothesis (in this case~$\cH_0$). 
Adding and subtracting~$\E[y_i|x_i]$ under square, we get
\begin{equation}
\label{eq:glm-decomposition}
\begin{aligned}
\wh S_0
= 
   \underbrace{\sum_{i=1}^{n} \frac{(y_i - \E[y_i|x_i])^2}{a''(\eta_{i}(\theta_1))} -  \nu(\theta_1)}_{\wh Q_0}
	&+ \underbrace{\frac{(a'(\eta_{i}(\theta_1)) - \E[y_i|x_i])^2}{a''(\eta_{i}(\theta_1))}}_{\wh R_0} 
%\\&    
    - \underbrace{\frac{2(a'(\eta_{i}(\theta_1)) - \E[y_i|x_i])(y_i - \E[y_i|x_i])}{a''(\eta_{i}(\theta_1))}}_{\wh U_0}.
\end{aligned}
\end{equation}
The term~$\wh Q_0$ corresponds to the centered~$\chi^2$-type statistic.
The term~$\wh R_0$ is non-random when conditioned on~$X = [x_1; ...; x_n],$ and incorporates the offset of the statistic due to~$\Delta^2$. 
The cross-term~$\wh U_0$ gives smaller-order fluctuations. 
Representing the ``unshifted'' term~$\wh S_1 = \wh S_0 - \wh S$ in a similar manner, where~$\wh S$ is the whole statistic whose sign is examined in~\eqref{eq:test-glm}, we decompose~$\wh S$ as follows:
\[
\wh S
= \wh S_0 - \wh S_1
= [\wh Q_0 - \wh Q_1] + [\wh R_0 - \wh R_1] + [\wh U_1 - \wh U_0].
\]
Here~$\wh Q_1, \wh R_1, \wh U_1$ are the counterparts of~$\wh Q_0, \wh R_0, \wh U_0$; we do not write them explicitly here.

\proofstep{1}.
For~$\wh Q_0 = \sum_{i=1}^n \xi_i^2 - n \nu(\theta_1)$ we have~$\E[\wh Q_0] = 0$ and
$
\Var[\wh Q_0] = \sum_{i=1}^n \Var[\xi_i^2] = n [\kappa(\theta_1) - \nu^2(\theta_1)],
$
where we used independence of~$\xi_i$'s. 
Hence, by Chebyshev's inequality
\[
\begin{aligned}
\Prob\left[  |\wh Q_0 | \le \frac{n \Delta^2}{c} \right] 
	&\ge 1-\frac{c^2 [\kappa(\theta_1) - \nu^2(\theta_1)]}{n \Delta^4},
\end{aligned}
\]
where~$c > 0$ will be chosen later. In particular, the probability in the right-hand side is~$\ge 0.975$ when
\[
n\Delta^4 \ge {40 c^2\kappa(\theta_1)}. 
\]
As a result, repeating the same analysis for~$\wh Q_1$, we get
\[
\Prob\left[  |\wh Q_0 - \wh Q_1| \le \frac{2n \Delta^2}{c} \right] \ge 0.95
\]
whenever 
\begin{equation}
\label{eq:n-kurtosis-apx}
n \ge \frac{40 c^2 \left[\kappa_0(\theta_1) \vee \kappa_1(\theta_1)\right]}{\Delta^4}.
\end{equation}
On the other hand, one may verify by straightforward numerical estimates that~\eqref{eq:n-kurtosis-apx} with~$c = 120$ is indeed implied by~\eqref{eq:condition_n}.

\proofstep{2}. 
Our next goal is to similarly bound~$\wh R_0 - \wh R_1$ as~$\Omega(n \Delta^2)$ with fixed probability.
To this end,
\[
\begin{aligned}
\wh R_0 
&= \sum_{i=1}^{n} \wh \Delta^2(x_i) + \frac{(a'(\eta_{i}(\theta_0)) - \E[y_i|x_i])^2}{a''(\eta_{i}(\theta_1))}
	+ 2\frac{a'(\eta_{i}(\theta_1)) - a'(\eta_{i}(\theta_0))}{\sqrt{a''(\eta_{i}(\theta_1))}} \cdot \frac{a'(\eta_{i}(\theta_0)) - \E[y_i|x_i]}{\sqrt{a''(\eta_{i}(\theta_1))}} \\
&\ge \sum_{i=1}^{n} \frac{\wh \Delta^2(x_i)}{2} - \frac{(a'(\eta_{i}(\theta_0)) - \E[y_i|x_i])^2}{a''(\eta_{i}(\theta_1))} 
= \sum_{i=1}^{n} \frac{\wh \Delta^2(x_i)}{2} - \Bias_0^2(\theta_1|x_i),
\end{aligned}
\]
where we introduced
\[
\wh\Delta^2(x) := \frac{[a'(\eta_x(\theta_k)) - a'(\eta_x(\theta_{1}))]^2}{a''(\eta_x(\theta_{1}))}
\]
and in the second line we used that~$-2ab \le a^2/2 + 2b^2$. 
Thus, we have
\[
\wh R_0  - \wh R_1 
\ge \sum_{i=1}^{n} \frac{\wh \Delta^2(x_i)}{2} - \Bias_0^2(\theta_1|x_i) - \Bias_1^2(\theta_1|\wt x_i).
\]
Now observe that, due to the small misspecification bias assumption~\eqref{eq:small-bias},
\[
\E\left[\sum_{i=1}^{n} \Bias_0^2(\theta_1|x_i) + \Bias_1^2(\theta_1|\wt x_i) \right] 
\le n(\Bias_0^2(\theta_1) + \Bias_1^2(\theta_1)) \le \frac{n\Delta^2}{400}.
\]
Hence, by Markov's inequality, 
\[
\Prob\left[\sum_{i=1}^{n} \Bias_0^2(\theta_1|x_i) + \Bias_1^2(\theta_1|\wt x_i) \le \frac{n\Delta^2}{40} \right] \ge 0.9. 
\]
On the other hand, by the Paley-Zygmund inequality~(\cite{paley1932note}), for arbitrary~$t \in [0,1]$ we have
\[
\Prob\left[\sum_{i=1}^{n} \wh \Delta^2(x_i) \ge t {n \Delta^2} \right] 
\ge (1-t)^2 \frac{n^2 \Delta^4}{\E\left[\left(\sum_{i=1}^{n} {\wh \Delta^2(x_i)}\right)^2\right]}.
\]
The denominator satisfies
\[
\E\left[\left(\sum_{i=1}^{n} {\wh \Delta^2(x_i)}\right)^2\right] 
= n \E[\wh \Delta^4] + n(n-1) \Delta^4 
= n^2 \Delta^4 + n \Var[\wh \Delta^2] 
\le \frac{81}{80} n^2 \Delta^4.
\]
where in the end we used that~$n \Delta^4 \ge 80 \Var[\wh \Delta^2]$, cf.~\eqref{eq:condition_n}. 
Thus, choosing~$t = 0.1,$ we arrive at
\[
\Prob\left[\sum_{i=1}^{n} \wh \Delta^2(x_i) \ge \frac{n \Delta^2}{10} \right]  \ge 0.8.
\]
Combining this with the previous result through the union bound, we get that
\[
\Prob\left[\wh R_0  - \wh R_1 \ge \frac{n \Delta^2}{40} \right]  \ge 0.7.
\]

\proofstep{3}.
It remains to upper-bound the cross-term~$\wh U_0-\wh U_1$. 
% The result is trivial if $\nu^2_{0}(\theta_{1}) = \kappa_{0}(\theta_{1})$ (since then the noise is deterministic conditionally on $X$), hence we assume that $\nu^2_{0}(\theta_{1}) \leq c \kappa_{0}(\theta_{1})$ for some $c \geq 1$.  The condition on $n$
% \[
% n \ge 
% \frac{20c^2}{\Delta^4}
% \max[\kappa_0(\theta_{1})-\nu_0^2(\theta_{1}),\kappa_{1}(\theta_{1})-\nu_{1}^2(\theta_{1})]
% \] 
First, note that condition~\eqref{eq:condition_n} implies
\begin{equation}
\label{eq:n-lower-bound-for-last-step}
\begin{aligned}
\sqrt{n}\Delta^{2} 
&\geq 40 c\sqrt{20\max \left[\kappa_{0}(\theta_{1}), \kappa_1(\theta_{1}), 4\E[\wh \Delta^4]\right]}\\
%\sqrt{n}\Delta^{2} &\geq 40c\sqrt{80 \E[\wh \Delta^4]}
\end{aligned}
\end{equation}
with~$c = 120$ (i.e., the same constant as in step~\proofstep{1}).
Now, consider the following event:
\[ 
\mathcal{E} = \left\{ \sum_{i=1}^n \hat{\Delta}^4(x_i) + \Bias_0^4(\theta_1|x_i) + \Bias_1^4(\theta_1|\wt x_i) \leq {10n\E[\wh\Delta^4]} \right\}.
\]
Using Markov's inequality and~\eqref{eq:small-bias}, one can verify that~$\Prob\left[ \mathcal{E} \right] \geq 0.98$.
Moreover,
\begin{align*}
\Prob\left[  |\wh U_0 - \wh U_1| \le \frac{n \Delta^2}{c} \right]  &\ge\Prob\left[ |\wh U_0 | + |\wh U_1 | \le \frac{n \Delta^2}{c} \right]  \\
& \ge\Prob\left[ |\wh U_0| \le \frac{n \Delta^2}{2c} \right] \Prob\left[ |\wh U_1 | \le \frac{n \Delta^2}{2c} \right] \\
&\ge \left(0.98 - \Prob\left[ |\wh U_0 |\ind_{\mathcal{E}} \ge \frac{n \Delta^2}{2c} \right] \right)\left(0.98 - \Prob\left[ |\wh U_1|\ind_{\mathcal{E}} \ge \frac{n \Delta^2}{2c} \right] \right)\\
	&\stackrel{(i)}{\ge} \left(0.98-\frac{16c^2 \E\left[\ind_{\mathcal{E}}\sum_{i=1}^n \alpha_{0}(\theta_1|x_i) \nu_0(\theta_1|x_i)\right]}{n^2 \Delta^4}\right)\\ 
	&\quad \times \left(0.98-\frac{16c^2 \E\left[\ind_{\mathcal{E}}\sum_{i=1}^n \alpha_{1}(\theta_1|\wt x_i) \nu_1(\theta_1|\wt x_i)\right]}{n^2 \Delta^4}\right)\\
	&\stackrel{(ii)}{\ge} \left( 0.98-\frac{16c^2 \E^{1/2}\left[\ind_{\mathcal{E}}\sum_{i=1}^n \alpha^2_{0}(\theta_1|x_i)\right]\sqrt{\kappa_{0}(\theta_1)}}{n^{3/2} \Delta^4}\right)\\
	&\quad \times \left( 0.98-\frac{16c^2 \E^{1/2}\left[\ind_{\mathcal{E}}\sum_{i=1}^n \alpha^2_{1}(\theta_1|\wt x_i)\right]\sqrt{\kappa_{1}(\theta_1)}}{n^{3/2} \Delta^4}\right) \\
	&\stackrel{(iii)}{\ge} \left(0.98 - \frac{64c^2\sqrt{10\kappa_1(\theta_1)\E[\wh\Delta^4]})}{n\Delta^4} \right) 
	\cdot \left(0.98 - \frac{16c^2\sqrt{10\kappa_0(\theta_1)\E[\wh\Delta^4]}}{n\Delta^4} \right)\\
	&\stackrel{(iv)}{\ge} 0.95, \;\; \text{where:}
\end{align*}
%Here we proceeded as follows:
\begin{itemize}
\item[-] in~$(i)$ we introduced the quantities~$\alpha^2_1(\theta_1|x) = \Bias_1^4(\theta_1|x)$ and
\[
\alpha^2_0(\theta_1|x):= \frac{(a'(\eta(\theta_1)) - \E[y|x])^4}{a''(\eta(\theta_1))^2} \leq 4 \hat{\Delta}^4(x) + 4
 \Bias_0^4(\theta_1|x),
 \] 
and then used Markov's inequality in the form~$\Prob[|X| \ge \varepsilon] \le \E[X^2]/\varepsilon^2$;
\item[-] in~$(ii)$ we used the Cauchy-Schwarz inequality first on the sum under the expectation to obtain the product of two random variables, and then used the Cauchy-Schwarz inequality again on the expectation of the product;
\item[-] in (iii) we used the definition of the event~$\mathcal{E}$;
\item[-] in (iv) we used~\eqref{eq:condition_n} and performed a direct calculation. 
\end{itemize}
Putting~$c = 120$, and combining the three bounds obtained in~\proofstep{1}--\proofstep{3} through the union bound, we bound the probability of type II error by~0.4 as required. 
\qed

\subsection{\odima{Adaptation for GLMs with small samples}}

Assume we can resample~$y$ for given~$x$, thus having two independent observations~$y,y'$. Under this assumption, we can consider an adaptive counterpart of test~\eqref{eq:test-glm}
\begin{equation}
\label{eq:test-glm-adapt}
\wh T = \ind\left\{
\sum_{i=1}^{n_0} \frac{(a_0'(\eta_{x_i}(\theta^*)) - y_i)^2}{a_0''(\eta_{x_i}(\theta^*))} - n_0 \wh\nu_0(\theta^*) 
\geq \sum_{i=1}^{n_1} \frac{(a_1'(\eta_{\wt x_i}(\theta^*)) - \wt y_i)^2}{a_1''(\eta_{\wt x_i}(\theta^*))} - n_1 \wh\nu_1(\theta^*) \right\},
\tag{$\texttt{\textup{GLM++}}$}
\end{equation}
where relative variances~$\nu_0(\theta^*),\nu_1(\theta^*)$ are replaced with the following estimates:
\[
\begin{aligned}
\wh\nu_0 = \frac{1}{2n_0} \sum_{i=1}^{n_0} \frac{(y_i - y_i')^2}{a_0''(\eta_{x_i}(\theta^*))}, 
\quad
\wh\nu_1 = \frac{1}{2n_1} \sum_{i=1}^{n_1} \frac{(\wt y_i - \wt y_i')^2}{a_1''(\eta_{\wt x_i}(\theta^*))}.
\end{aligned}
\]
Here~$(y_i,y_i')$ and~$\wt y_i, \wt y_i'$ are obtained through conditional resampling as explained above. 
Note that, using~\eqref{eq:glm-loss-derivatives}, and recalling that we have~$n_{k} \le r_k$, we can rewrite these estimates as
\[
\wh \nu_{k} = \frac{1}{2} \|\wh \H_{k}(\theta^*)^{\pinv/2}[\nabla \wh L_k(\theta^*) - \nabla \wh L_k'(\theta^*)]\|^2 \quad (k \in \{0,1\}),
\]
where~$\wh L_k'(\theta^*)$ is empirical risk computed with resampled responses. 
Clearly,~$\wh \nu_k$ these estimates are unbiased over the joint expectations over~$(X,Y,Y')$ and~$(\wt X,\wt Y,\wt Y')$.
Now, observe that, when analyzing the error probabilities for test~\eqref{eq:test-glm-adapt}, we can decompose the statistic almost in the same way as for~\eqref{eq:test-glm}, with two additional terms corresponding to the fluctuations of~$\wh \nu_0, \wh \nu_1$ around their expectations. More precisely, representing~$\wh S = \wh S_0 - \wh S_1$ as in the proof of Theorem~\ref{th:glm-fixed-prob}, the decomposition of~$\wh S_0$ for the new test becomes
\[
\wh S_0 = \wh Q_0 + \wh R_0 - \wh U_0 - \wh V_0 \;\; \text{with} \;\; \wh V_0 := n_0 (\wh \nu_0 - \nu_0(\theta^*)),
\]
where the first three terms are the same as in~\eqref{eq:glm-decomposition}. Thus, introducing~$\wh V_1 := n_1 (\nu_1(\theta^*) - \wh \nu_1)$, we have
\[
\wh S
= [\wh Q_0 - \wh Q_1] + [\wh R_0 - \wh R_1] + [\wh U_1 - \wh U_0] + [\wh V_1 - \wh V_0]. 
\]
Let us now show that the additional fluctuation term~$|\wh V_1 - \wh V_0|$ in the above decomposition admits the same bound as the term~$|\wh U_0 - \wh U_1|$. 
%(this will give the final result up to a change in constants.) 
Indeed, in the notation of the proof of Theorem~\ref{th:glm-fixed-prob}, by Chebyshev's inequality we have
\[
\begin{aligned}
\Prob\left[ |\wh V_0| \ge \frac{n\Delta^2}{c} \right] 
\le \frac{c^2 \Var[n\wh\nu_0]}{n^2 \Delta^4} 
= \frac{c^2}{n \Delta^4} \Var\left[\frac{(y - y')^2}{2a_1''(\eta_{x}(\theta^*))} \right]
= \frac{c^2}{n \Delta^4} \left( \E\left[\frac{(y - y')^4}{4a_1''(\eta_{x}(\theta^*))^2}\right] - \nu_0(\theta^*) \right).
\end{aligned}
\]
Furthermore, 
\[
\E\left[\frac{(y - y')^4}{4a_1''(\eta_{x}(\theta^*))^2}\right] 
= \E\left[\frac{(y - \E[y|x] - (y' - \E[y'|x]) )^4}{4a_1''(\eta_{x}(\theta^*))^2}\right];
\]
thus, for independent~$\xi = y - \E[y|x]$ and~$\xi' = y' - \E[y|x]$ such that~$\E[\xi|x] = \E[\xi'|x] = 0$, we have
\[
\E\left[\frac{(y - y')^4}{4a_1''(\eta_{x}(\theta^*))^2}\right] 
= \E\left[\frac{\E[(\xi - \xi')^4|x]}{4a_1''(\eta_{x}(\theta^*))^2}\right] 
= \E\left[\frac{\E[\xi^4|x]}{2a_1''(\eta_{x}(\theta^*))^2}\right] 
	+ \E\left[\frac{3(\E[\xi^2|x])^2}{2a_1''(\eta_{x}(\theta^*))^2}\right]
= \frac{\kappa_0(\theta^*)}{2} + \frac{3\nu_0^2(\theta^*)}{2}.
\]
As a result,
\[
\Prob\left[ |\wh V_0| \ge \frac{n\Delta^2}{c} \right] 
\le \frac{c^2(\kappa_0(\theta^*) + \nu_0^2(\theta^*))}{2n\Delta^4} 
\le \frac{c^2\kappa_0(\theta^*)}{n\Delta^4}.
\]
We see that, under~\eqref{eq:n-kurtosis-apx} (assuming hypothesis~$\cH_1$ w.l.o.g.) the bound~$|\wh V_0 - \wh V_1| \le 2n\Delta^2/c$ holds with fixed probability. 
Repeating steps~\proofstep{1}-\proofstep{3} in the proof of Theorem~\ref{th:glm-fixed-prob}, we obtain the same result.
\qed

\section{Suboptimality of test~\eqref{eq:test_grad}}
\label{app:grad}

For simplicity, we let~$n_0 = n_1 = n$ and consider the setup of a well-specified linear model with fixed design (cf.~Sec.~\ref{sec:gaussian}); the example can easily be extended for  random design.
Recall that, by Proposition~\ref{prop:upper-fixed-design}, our proposed test~\eqref{eq:test_1} has type I error probability
\[
\Prob_{\cH_0}[\hat{T} = 1|X, \wt X] \le C \exp \left(-c n_1^{\vphantom 2} \wh\Delta_1^2  \min\left[1, \frac{n_1^{\vphantom 2}\wh\Delta_1^2}{\wh r} \right]\right),
\]
and a similar bound for type II error (with the replacement~$1 \mapsto 0$ of the subscript). 
Here, the (empirical) separation measures~$\wh\Delta_0^2,\wh\Delta_1^2$ are given by
\[
\wh\Delta_0^2 = \|\wh\bSigma_0^{1/2}(\theta_1 - \theta_0)\|^2,
\quad
\wh\Delta_1^2 = \|\wh\bSigma_1^{1/2}(\theta_1 - \theta_0)\|^2,
\]
%we have, under the Gaussian linear model with fixed design, that 
%as shown by the following result.
and~$\wh r = \max[\wh r_0, \wh r_1]$, where~$\wh r_k = \rank(\wh\bSigma_k)$.
 %\rank(\wh \bSigma_0) \vee \rank(\wh \bSigma_1) $,
%and $\hat{T}$ defined in \eqref{eq:test_1}. 
We now construct a problem instance in which the gradient test~$\wh T'$, given by~\eqref{eq:test_grad}, is suboptimal.
To this end, let~$\wh \bSigma_0$ and~$\wh \bSigma_1$ have the same rank~$\wh r$, smallest non-zero eigenvalue~$1/\kappa$ and other eigenvalues equal to~$1$, for~$\kappa > 0$ to be fixed later. 
%W.l.o.g., let us assume that the smallest eigenvalue of~$\wh\bSigma_1$ is not greater than that of~$\wh \bSigma_0$, 
Now, let us take~$\theta_1 - \theta_0$ as the unit vector in the direction corresponding to the smallest eigenvalue of~$\wh \bSigma_1$. 
Then,~$\wh \Delta_1^2 = {1}/{\kappa} \le \wh \Delta_0^2.$
On the other hand, the quantities~$\wh \delta_k^2 := \|\wh\bSigma_k(\theta_1 - \theta_0)\|^2$,~$k \in \{0,1\}$, satisfy
\[
\wh \delta_1^2 = \frac{\wh \Delta_1^2}{\kappa} = \frac{1}{\kappa^2} \le \wh \delta_0^2.
\]
Now, observe that~$\wh\delta_1^2$ controls the sum of errors of the gradient norm test~\eqref{eq:test_grad} in a similar manner as~$\wh\Delta_1^2$ controls that for test~\eqref{eq:test_1}. Indeed, proceeding as in the proof of Proposition~\ref{prop:upper-fixed-design}, we have
\[
\begin{aligned}
&\Prob_{\cH_0}[\wh T'=1 | X,\wt X] \\
&= \Prob \left[ 
\underbrace{\tfrac{1}{n}\| X^{\top}\xi\|^2 - \E[\tfrac{1}{n}\| X^{\top}\xi\|^2|X]}_{U}  
+ 
\underbrace{\E[\tfrac{1}{n}\|\wt X^\top \wt \xi\|^2|\wt X] - \tfrac{1}{n} \|\wt X^\top \wt \xi\|^2}_{V}    
+ 
\underbrace{2\langle \wh \bSigma_1 (\theta_1 - \theta_0),\tilde{X}^\top\tilde{\xi} \rangle}_{W} \geq n \wh \delta_1^2 \right].
\end{aligned}
\]
As our goal is to show suboptimality, let us bound~$\Prob_{\cH_0}[\wh T'=1 | X,\wt X]$ from below. Since~$\tfrac{1}{n}XX^\top$ has the same eigenvalues as~$\wh \bSigma_0 = \frac{1}{n}X^\top X$, and similarly for~$\frac{1}{n}\wt X \wt X^\top$, we have that~$\tfrac{1}{n}\| X^{\top}\xi\|^2$ is distributed as~$\frac{1}{\kappa}\zeta^2 + \chi_{\wh r-1}^2$, where~$\chi_{\wh r-1}^2$ is chi-squared with~$\wh r-1$ degrees of freedom, and~$\zeta \sim \cN(0,1)$ is independent from~$\chi_{\wh r-1}^2.$ 
Thus, we estimate the (conditional to~$X$) variance of~$U$ above as
\[
\Var[U|X] \le \wh r( \wh r-1) + 3\wh r - (\wh r-1)^2 \le 4\wh r,
\]
where we used that~$\E[\zeta^4] = 3$. Similarly,~$\Var[V|\wt X] \le 4 \wh r$. Finally, by the definition of~$\theta_1 - \theta_0$ we find 
\[
\Var[W|\wt X] = 4 \| \wt X \wh\bSigma_1(\theta_1 - \theta_0)\|^2 
= \frac{4}{\kappa^2} \|\wt X (\theta_1 - \theta_0)\|^2
= \frac{4n \wh\Delta_1^2}{\kappa^2} = \frac{4n \wh\delta_1^2}{\kappa}. 
\]
Thus,
\[
\Var[\tfrac{1}{\kappa} \zeta^2 - \tfrac{1}{\kappa} + V + W] 
\le \Var[U + V + W] 
\le 3\left(8\wh r + \frac{4n\wh\delta_1^2}{\kappa} \right). 
\]
By Chebyshev's inequality, any centered random variable~$Z$ satisfies
$
\Prob[Z \le 2\sqrt{\Var[Z]}] \ge 1/2. 
$
Applying this to~$Z =\tfrac{1}{\kappa} \zeta^2 - \tfrac{1}{\kappa} + V + W$, we arrive at
\[
\begin{aligned}
\Prob_{\cH_0}[\wh T'=1 | X,\wt X] 
&\ge \frac{1}{2} \Prob\left[\chi_{\wh r-1}^2 - (\wh r-1) \ge n\wh\delta_1^2 - 10\left(\sqrt{\wh r + \frac{n\wh\delta_1^2}{\kappa}}\right)\right] \\
&\ge \frac{1}{2} \Prob\left[\chi_{\wh r-1}^2 - (\wh r-1) \ge \frac{1}{\kappa} \left( n\wh\Delta_1^2- 10\sqrt{\kappa^2 \wh r + n\wh\Delta_1^2}\right)\right] 
\end{aligned}
\]
Now, for~$\wh r$ large enough, consider the regime
\begin{equation}
\label{eq:hard-range}
40\sqrt{\wh r} \le \frac{n\wh\Delta_1^2}{\kappa} \le 3\wh r  
\quad \iff \quad
40\sqrt{\wh r} \le \frac{n}{\kappa^2} \le 3\wh r.
\end{equation}
By simple algebra, the expression in parentheses in this regime is at most~$n\wh\Delta_1^2/(2\kappa)$, thus, 
\[
\Prob_{\cH_0}[\wh T'=1 | X,\wt X]  
\ge \frac{1}{2} \Prob\left[\chi_{\wh r-1}^2 - (\wh r-1) \ge \frac{n\wh\Delta_1^2}{2\kappa} \right].
\]
On the other hand, in this regime we can apply the lower bound for the right tail probability of the chi-squared distribution (cf.~\eqref{eq:chi-squared-lower-estimates}), which gives
\[
\Prob_{\cH_0}[\wh T'=1 | X,\wt X]  
\ge c\exp\left( -\frac{C}{\kappa^2} \frac{n^2\wh\Delta_1^4}{\wh r}\right).
\]
Now, allowing~$\wh r$ to grow, let us put~$\kappa = \sqrt{\wh r}$ and~$n = 40\wh r^{3/2}$ 
(this is on ``the left edge'' of~\eqref{eq:hard-range}). Then, 
\[
\Prob_{\cH_0}[\wh T'=1 | X,\wt X]  \ge c.
\]
On the other hand, in this regime we have~$n\wh\Delta_1^2 \asymp \wh r$ up to a constant, whence, returning to test~\eqref{eq:test_1}, 
\[
\Prob_{\cH_0}[\hat{T} = 1|X, \wt X] + \Prob_{\cH_1}[\hat{T} = 0|X, \wt X] 
\le C \exp \bigg(-\frac{cn^2\wh\Delta_1^4}{\wh r}\bigg) \le C\exp(-c\wh r).
\]
Thus, there is a widening gap (as~$\wh r$ grows) between the error bounds for the tests~$\wh T$ and~$\wh T'$ (and moreover,~$\wh T'$ is not even consistent in this regime, whereas~$\wh T$ still is).
\qed

%%%%%%%%%%%%%%%%%%%%%%%%%%%%%%%%%%%%%%%%%%%%%%%%%%%%%%%%%%%%

\section{Remaining proofs}

\subsection{Verification of~\eqref{eq:complexity-gaussian}}  %sample complexity bound

W.l.o.g., let~$\Delta_0^2 = \Delta_1^2 = \Delta^2$ and~$n_0 = n_1 = n$ (the general case is similar). Recall that~$\Delta^2 \le 1$. Moreover,~$r = \max[r_0, r_1]$ and we also denote~$\wh r = \min(r,n)$. 
We now prove that~\eqref{eq:complexity-gaussian} is equivalent to
\begin{equation}
\label{eq:upper-random-design-log}
n^{\vphantom 2} \Delta^2 \min\left[1,\frac{n^{\vphantom 2}\Delta^2}{\wh r}\right] \ge c,
\end{equation}
up to a change in the constant~$c \ge 1$. 
(According to~\eqref{eq:upper-random-design}, this would allow to bound the probabilities of error of both types with~$2Ce^{-c}$.) 
Indeed, taking the second term in the minimum in~\eqref{eq:upper-random-design-log}, we get
\[
n \Delta^2 \ge \sqrt{c \, \wh r} = \sqrt{c \min[r,n]},
\]
whence
\[
n \ge \min\left[ \frac{c}{\Delta^4}, \frac{\sqrt{c\, r}}{\Delta^2} \right],
\]
which is nothing but~\eqref{eq:complexity-gaussian}, up to the replacement~$c \mapsto \sqrt{c}$ (we can w.l.o.g.~assume~$c \ge 1$). 
Thus,~\eqref{eq:upper-random-design-log} indeed implies~\eqref{eq:complexity-gaussian} with a change of constant.

Conversely,~\eqref{eq:complexity-gaussian} is  equivalent to
\[
n\Delta^2 \ge c\min\left[\frac{1}{\Delta^2}, \sqrt{r} \right]. %= \frac{c}{\Delta^2}.
\]
On the other hand,~\eqref{eq:upper-random-design-log} is equivalent to 
\[
n\Delta^2 
\ge c\max\left[1, \frac{\wh r}{n\Delta^2} \right] 
= c \max\left[1, \min\left[\frac{1}{\Delta^2}, \frac{r}{n\Delta^2}\right]\right]
= c \min\left[\frac{1}{\Delta^2}, \max\left[1, \frac{r}{n\Delta^2}\right]\right],
\]
where in the last step we used~$\Delta^2 \le 1$. Thus, the first case for the minimum in~\eqref{eq:complexity-gaussian} is identical to the first case for the minimum in~\eqref{eq:upper-random-design-log}. On the other hand, the second case in~\eqref{eq:complexity-gaussian} clearly implies~$n\Delta^2 \ge c$ and~$n^2\Delta^4 \ge c^2r$, i.e., the second case in~\eqref{eq:upper-random-design-log} up to a change of constant.
Thus,~\eqref{eq:complexity-gaussian} implies~\eqref{eq:upper-random-design-log}.
%where the inequality is equivalent to~\eqref{eq:complexity-gaussian}, and the equality follows from~$\Delta^2 \ge 1/\sqrt{r}$. 
%Bounding~$\Delta^2 \le 1$, we have~$n\Delta^2 \ge c$, which is the first requiment in~\eqref{eq:upper-random-design-log}. 
%On the other hand, we also have~$n\Delta^4 \ge c,$ whence~$n^2\Delta^4 \ge cn \ge c\bar r,$
%which is the second requirement in~\eqref{eq:upper-random-design-log}.
\qed

\subsection{Verification of~\eqref{eq:chi-square-with-resampling}}
Observe that~$\xi' = \tfrac{1}{\sigma_0} (Y' - X'^\top \theta_0)$ and~$\xi'' = \tfrac{1}{\sigma_0} (Y'' - X''^\top \theta_0)$ are independent samples from~$\cN(0,\Id_{n})$. 
Moreover, \odima{mistake with projector!}
\[
\begin{aligned}
%\Big[\wh\bSigma_0'^{\pinv} + \wh\bSigma_0''^{\,\pinv} \Big]^{\pinv/2} 
\wh\bSigma_0'^{\pinv} X'^\top Y' -\wh\bSigma_0''^{\,\pinv} X''^\top Y'' 
%\Big[\wh\bSigma_0^{\pinv} + \wh\bSigma_0'^{\,\pinv} \Big]^{\pinv/2} \\
&= \wh\bSigma_0'^{\pinv} X'^\top (Y'-X'\theta_0) -\wh\bSigma_0''^{\,\pinv} X''^\top (Y''-X''\theta_0) \\
&= \sigma_0 \big(\wh\bSigma_0'^{\pinv} X'^\top \xi' -\wh\bSigma_0''^{\,\pinv} X''^\top \xi''\big)\\
&= \sqrt{n}\sigma_0 \big(\wh\bSigma_0'^{\pinv/2} \zeta' + \wh\bSigma_0''^{\,\pinv/2} \zeta''\big)
\sim \sqrt{n}\sigma_0 \cdot \cN(0,\wh\bSigma_0'^{\pinv} + \wh\bSigma_0''^{\pinv}).
\end{aligned} 
\]
Here~$\zeta'$ and~$\zeta''$ are independent samples from~$\cN(0,\Id_{\wh r_0})$, and~$\rank(\wh\bSigma_0'^{\pinv} + \wh\bSigma_0''^{\pinv}) = \rank(\wh\bSigma_0') + \rank(\wh\bSigma_0'') = 2\wh r_0$ a.s., since~$\wh\bSigma_0'$ and~$\wh\bSigma_0''$ are PSD. \odima{check this!}
Returning to~\eqref{eq:resampling-trick}, we see that the corresponding statistic is indeed distributed as~$\chi_{2\wh r_0}^2/(2\wh r_0)$. 
\qed

\subsection{Proof of Proposition~\ref{prop:upper-fixed-design-adapt}: remaining term}

Recall that it only remains to estimate the fourth term in the right-hand side of~\eqref{eq:gaussian-adapt-expansion}.
We use that~$\Prob[\wh \tau_1 \ge 2] \le 2\exp(-cn)$ by~\eqref{eq:var-ratio-tail-bound}, and~$\wh \tau_0$ is (conditionally) independent from~$\wh \tau_1$:
\[
\begin{aligned}
\Prob \bigg[ \wh \tau_1 \bigg(\frac{1}{\wh \tau_0} - 1\bigg) \ge \frac{n \wh\Delta_1^2}{5 \wh r_0 \sigma_1^2} \bigg]	
&\le 
2\exp(-cn) + \Prob \bigg[ \bigg(\frac{1}{\wh \tau_0} - 1\bigg) \ge \frac{n \wh\Delta_1^2}{10 \wh r_0 \sigma_1^2} \bigg] \\
&\le 
2\exp(-cn) + \Prob \bigg[ \wh \tau_0 \le 1 - \frac{1}{2}\min \bigg[ \frac{n \wh\Delta_1^2}{10 \wh r_0 \sigma_1^2}, 1\bigg] \bigg] \\
&\le 
4\exp(-c_4 n) + 2\exp \bigg( - \frac{c_4 n \wh \Delta_1^2}{\sigma_1^2} \min\bigg[1, \frac{n \wh \Delta_1^2}{\wh r_0 \sigma_1^2}\bigg] \bigg).
\end{aligned}
\]
Here we used that~$\tfrac{1}{1+t} \le 1-\tfrac{1}{2}\min[t,1]$ for~$t \ge 0$ and proceeded via~\eqref{eq:var-ratio-tail-bound} as when dealing with the third term in the right-hand side of~\eqref{eq:gaussian-adapt-expansion}.
\qed

%For the last term we have
%\[
%\begin{aligned}
%\Prob \bigg[ \frac{\wh\tau_1}{\wh \tau_0} (\| \xi\|^2_X - \wh r_0) \geq \frac{n \wh\Delta_1^2}{5 \sigma_1^2}\bigg] 
%%&\le 2\exp(-cn) + \Prob \bigg[ \frac{1}{\wh \tau_0} (\| \xi\|^2_X - \wh r_0) \geq \frac{n \wh\Delta_1^2}{5 \sigma_1^2}\bigg] \\
%&\le 4\exp(-cn) + \Prob \bigg[ \| \xi\|^2_X - \wh r_0 \geq \frac{n \wh\Delta_1^2}{5 \sigma_1^2}\bigg] \\
%&\le  4\exp(-cn) + \exp\bigg(-\frac{c_5 n \wh\Delta_1^2}{\sigma_1^2} \min\bigg[1, \frac{n \wh\Delta_1^2}{\wh r_0 \sigma_1^2}\bigg]\bigg),
%\end{aligned}
%\]
%where we used that~$\wh \tau_1,$~$\wh \tau_0$ and~$\| \xi\|^2_X - \wh r_0$ are conditionally independent and concluded via~\eqref{eq:tail-bounds}. 

\subsection{Proof of Corollary \ref{cor:voting}}
By Theorem \ref{th:glm-fixed-prob}, we have that~$\Prob_{0}[\wh T_j = 1] \le 0.4$ for all $j \in [k]$. 
Hence
\begin{align*} 
\Prob_{\cH_0}[\wh T = 1] &= \Prob_{\cH_0}\bigg[ \sum_{j=1}^k \hat{T}_j \geq 0.5 k \bigg]
\leq \Prob_{\cH_0}\bigg[ \sum_{j=1}^k \hat{T}_j - \E_0[\hat{T}_j] \geq 0.1 k\bigg]
\leq  e^{-ck},
\end{align*}
for some constant $c>0$, where the final transition is by Hoeffding's inequality. Using~\eqref{eq:choose_k}, we get
\[
\Prob_{\cH_0}[\wh T = 1] \le \exp\bigg(-c'n\min\bigg[\frac{\Delta^4}{\kappa_{0}(\theta_{1})+\kappa_{1}(\theta_1)},1\bigg]\bigg).
\]
for $c'>0$. A similar result holds for $\Prob_{\cH_1}[\wh T = 0]$ by symmetry.
\qed

\end{document}
